# Supplementary material for: Nonlocal van der Waals functionals for solids: Choosing an appropriate one
Source: arXiv:1903.00284 ancillary file (2019-06-05)
Supplement: Supplementary file 1 [file Supplemental_Material.pdf]

# Supplemental Material

## Nonlocal van der Waals functionals for solids: Choosing an appropriate one

Fabien Tran,[1] Leila Kalantari,[1] Boubacar Traoré,[2] Xavier Rocquefelte,[3] and Peter Blaha[1]

[1] *Institute of Materials Chemistry, Vienna University of Technology, Getreidemarkt 9/165-TC, A-1060 Vienna, Austria*

[2] *Univ Rennes, INSA Rennes, CNRS, Institut FOTON - UMR 6082, F-35000 Rennes, France*

[3] *Univ Rennes, ENSCR, INSA Rennes, CNRS, ISCR (Institut des Sciences Chimiques de Rennes) - UMR 6226, F-35000 Rennes, France*

TABLE S1. Equilibrium lattice constant $a_0$ (in Å) of 44 solids. All results were obtained non-self-consistently using PBE orbitals/density. The space group number is indicated in parenthesis.

| Solid | Expt. | TM | SCAN | PBEsol | PBE | LDA | SCAN+rVV10 | PBEsol+rVV10s | C09-vdW |
|---|---|---|---|---|---|---|---|---|---|
| C (227) | 3.553 | 3.555 | 3.556 | 3.557 | 3.575 | 3.536 | 3.554 | 3.556 | 3.562 |
| Si (227) | 5.412 | 5.416 | 5.434 | 5.434 | 5.471 | 5.402 | 5.428 | 5.426 | 5.432 |
| Ge (227) | 5.641 | 5.651 | 5.670 | 5.679 | 5.764 | 5.626 | 5.657 | 5.668 | 5.684 |
| Sn (227) | 6.477 | 6.527 | 6.552 | 6.543 | 6.657 | 6.478 | 6.529 | 6.523 | 6.541 |
| SiC (216) | 4.346 | 4.353 | 4.360 | 4.362 | 4.385 | 4.335 | 4.357 | 4.359 | 4.363 |
| BN (216) | 3.592 | 3.610 | 3.607 | 3.610 | 3.628 | 3.585 | 3.605 | 3.608 | 3.613 |
| BP (216) | 4.525 | 4.514 | 4.529 | 4.522 | 4.550 | 4.493 | 4.525 | 4.517 | 4.528 |
| AlN (216) | 4.368 | 4.379 | 4.370 | 4.383 | 4.408 | 4.349 | 4.366 | 4.379 | 4.380 |
| AlP (216) | 5.451 | 5.462 | 5.482 | 5.476 | 5.513 | 5.440 | 5.475 | 5.469 | 5.473 |
| AlAs (216) | 5.649 | 5.661 | 5.682 | 5.681 | 5.735 | 5.636 | 5.673 | 5.674 | 5.679 |
| GaN (216) | 4.509 | 4.506 | 4.499 | 4.503 | 4.551 | 4.463 | 4.493 | 4.498 | 4.505 |
| GaP (216) | 5.439 | 5.434 | 5.446 | 5.442 | 5.508 | 5.395 | 5.436 | 5.431 | 5.446 |
| GaAs (216) | 5.640 | 5.643 | 5.664 | 5.663 | 5.749 | 5.607 | 5.650 | 5.651 | 5.668 |
| InP (216) | 5.858 | 5.884 | 5.898 | 5.882 | 5.961 | 5.831 | 5.884 | 5.865 | 5.883 |
| InAs (216) | 6.047 | 6.082 | 6.097 | 6.089 | 6.187 | 6.029 | 6.079 | 6.073 | 6.090 |
| InSb (216) | 6.473 | 6.516 | 6.534 | 6.521 | 6.636 | 6.453 | 6.511 | 6.500 | 6.519 |
| LiH (225) | 3.979 | 3.938 | 3.995 | 3.981 | 4.008 | 3.914 | 3.990 | 3.978 | 4.012 |
| LiF (225) | 3.972 | 3.973 | 3.986 | 4.009 | 4.070 | 3.915 | 3.974 | 3.996 | 4.016 |
| LiCl (225) | 5.070 | 5.050 | 5.096 | 5.065 | 5.152 | 4.966 | 5.073 | 5.041 | 5.069 |
| NaF (225) | 4.582 | 4.590 | 4.577 | 4.634 | 4.706 | 4.510 | 4.562 | 4.613 | 4.630 |
| NaCl (225) | 5.569 | 5.567 | 5.593 | 5.607 | 5.700 | 5.468 | 5.565 | 5.572 | 5.589 |
| MgO (225) | 4.189 | 4.218 | 4.204 | 4.220 | 4.259 | 4.167 | 4.199 | 4.214 | 4.214 |
| Li (229) | 3.443 | 3.403 | 3.471 | 3.435 | 3.437 | 3.365 | 3.469 | 3.431 | 3.462 |
| Na (229) | 4.205 | 4.131 | 4.205 | 4.172 | 4.200 | 4.054 | 4.194 | 4.157 | 4.190 |
| Al (225) | 4.022 | 3.986 | 4.012 | 4.015 | 4.041 | 3.983 | 4.009 | 4.010 | 4.019 |
| K (229) | 5.246 | 5.210 | 5.341 | 5.216 | 5.283 | 5.044 | 5.309 | 5.178 | 5.208 |
| Ca (225) | 5.559 | 5.494 | 5.555 | 5.456 | 5.527 | 5.333 | 5.540 | 5.440 | 5.435 |
| Rb (229) | 5.629 | 5.575 | 5.690 | 5.570 | 5.671 | 5.373 | 5.644 | 5.523 | 5.522 |
| Sr (225) | 6.059 | 5.972 | 6.077 | 5.917 | 6.024 | 5.785 | 6.048 | 5.893 | 5.885 |
| Cs (229) | 6.043 | 6.084 | 6.272 | 6.010 | 6.162 | 5.753 | 6.195 | 5.920 | 5.876 |
| Ba (229) | 4.994 | 4.967 | 5.042 | 4.879 | 5.020 | 4.750 | 5.000 | 4.847 | 4.833 |
| V (229) | 3.023 | 2.982 | 2.966 | 2.960 | 2.998 | 2.927 | 2.961 | 2.955 | 2.958 |
| Ni (225) | 3.510 | 3.465 | 3.456 | 3.462 | 3.518 | 3.423 | 3.449 | 3.452 | 3.464 |
| Cu (225) | 3.599 | 3.559 | 3.559 | 3.567 | 3.632 | 3.522 | 3.551 | 3.556 | 3.570 |
| Nb (229) | 3.300 | 3.292 | 3.294 | 3.272 | 3.312 | 3.246 | 3.288 | 3.268 | 3.272 |
| Mo (229) | 3.142 | 3.142 | 3.143 | 3.130 | 3.162 | 3.112 | 3.139 | 3.127 | 3.131 |
| Rh (225) | 3.786 | 3.792 | 3.783 | 3.783 | 3.832 | 3.756 | 3.776 | 3.776 | 3.784 |
| Pd (225) | 3.876 | 3.890 | 3.888 | 3.876 | 3.943 | 3.840 | 3.877 | 3.865 | 3.877 |
| Ag (225) | 4.070 | 4.069 | 4.084 | 4.053 | 4.148 | 4.001 | 4.067 | 4.038 | 4.053 |
| Ta (229) | 3.298 | 3.290 | 3.274 | 3.281 | 3.320 | 3.252 | 3.268 | 3.276 | 3.279 |
| W (229) | 3.162 | 3.158 | 3.149 | 3.155 | 3.185 | 3.136 | 3.145 | 3.151 | 3.156 |
| Ir (225) | 3.831 | 3.835 | 3.802 | 3.833 | 3.873 | 3.813 | 3.797 | 3.827 | 3.836 |
| Pt (225) | 3.917 | 3.921 | 3.907 | 3.919 | 3.971 | 3.895 | 3.899 | 3.910 | 3.922 |
| Au (225) | 4.067 | 4.091 | 4.093 | 4.084 | 4.161 | 4.048 | 4.080 | 4.073 | 4.088 |
| ME | | -0.006 | 0.018 | -0.005 | 0.056 | -0.071 | 0.004 | -0.019 | -0.009 |
| MAE | | 0.023 | 0.030 | 0.030 | 0.061 | 0.071 | 0.022 | 0.034 | 0.037 |
| MRE | | -0.2 | 0.3 | -0.1 | 1.1 | -1.5 | -0.0 | -0.4 | -0.2 |
| MARE | | 0.5 | 0.6 | 0.6 | 1.2 | 1.5 | 0.5 | 0.7 | 0.8 |

TABLE S2. Equilibrium lattice constant $a_0$ (in Å) of 44 solids. All results were obtained non-self-consistently using PBE orbitals/density. The space group number is indicated in parenthesis.

| Solid | vdW-DF-cx | PBE-D3(BJ) | optB86b-vdW | PBE+rVV10L | rev-vdW-DF2 | revPBE-D3(BJ) | optB88-vdW | rVV10 |
|---|---|---|---|---|---|---|---|---|
| C (227) | 3.567 | 3.563 | 3.571 | 3.571 | 3.569 | 3.560 | 3.576 | 3.585 |
| Si (227) | 5.441 | 5.426 | 5.451 | 5.458 | 5.453 | 5.397 | 5.464 | 5.485 |
| Ge (227) | 5.696 | 5.709 | 5.724 | 5.736 | 5.736 | 5.689 | 5.761 | 5.808 |
| Sn (227) | 6.557 | 6.582 | 6.593 | 6.611 | 6.611 | 6.564 | 6.637 | 6.684 |
| SiC (216) | 4.369 | 4.358 | 4.374 | 4.379 | 4.374 | 4.343 | 4.380 | 4.400 |
| BN (216) | 3.620 | 3.614 | 3.622 | 3.624 | 3.621 | 3.609 | 3.626 | 3.640 |
| BP (216) | 4.536 | 4.515 | 4.542 | 4.542 | 4.541 | 4.492 | 4.553 | 4.566 |
| AlN (216) | 4.389 | 4.381 | 4.391 | 4.401 | 4.392 | 4.370 | 4.394 | 4.416 |
| AlP (216) | 5.484 | 5.463 | 5.491 | 5.500 | 5.494 | 5.433 | 5.502 | 5.522 |
| AlAs (216) | 5.691 | 5.677 | 5.704 | 5.716 | 5.709 | 5.647 | 5.720 | 5.757 |
| GaN (216) | 4.513 | 4.525 | 4.527 | 4.539 | 4.531 | 4.519 | 4.543 | 4.576 |
| GaP (216) | 5.457 | 5.454 | 5.478 | 5.487 | 5.484 | 5.428 | 5.504 | 5.528 |
| GaAs (216) | 5.680 | 5.686 | 5.708 | 5.720 | 5.718 | 5.659 | 5.741 | 5.783 |
| InP (216) | 5.896 | 5.901 | 5.920 | 5.932 | 5.929 | 5.878 | 5.952 | 5.978 |
| InAs (216) | 6.104 | 6.118 | 6.135 | 6.150 | 6.148 | 6.094 | 6.173 | 6.214 |
| InSb (216) | 6.536 | 6.552 | 6.571 | 6.589 | 6.587 | 6.527 | 6.613 | 6.654 |
| LiH (225) | 4.052 | 3.897 | 4.019 | 3.998 | 4.013 | 3.818 | 4.011 | 4.004 |
| LiF (225) | 4.056 | 4.013 | 4.037 | 4.047 | 4.039 | 4.015 | 4.033 | 4.032 |
| LiCl (225) | 5.110 | 5.050 | 5.101 | 5.106 | 5.105 | 5.020 | 5.112 | 5.106 |
| NaF (225) | 4.689 | 4.644 | 4.652 | 4.673 | 4.656 | 4.675 | 4.641 | 4.638 |
| NaCl (225) | 5.661 | 5.595 | 5.619 | 5.642 | 5.625 | 5.604 | 5.614 | 5.601 |
| MgO (225) | 4.231 | 4.220 | 4.230 | 4.246 | 4.232 | 4.209 | 4.232 | 4.257 |
| Li (229) | 3.497 | 3.335 | 3.453 | 3.433 | 3.441 | 3.279 | 3.433 | 3.411 |
| Na (229) | 4.258 | 4.092 | 4.188 | 4.180 | 4.181 | 4.085 | 4.165 | 4.133 |
| Al (225) | 4.029 | 3.988 | 4.032 | 4.034 | 4.037 | 3.956 | 4.049 | 4.027 |
| K (229) | 5.310 | 5.168 | 5.218 | 5.228 | 5.220 | 5.221 | 5.184 | 5.136 |
| Ca (225) | 5.471 | 5.442 | 5.459 | 5.498 | 5.461 | 5.445 | 5.444 | 5.456 |
| Rb (229) | 5.615 | 5.559 | 5.544 | 5.589 | 5.558 | 5.650 | 5.512 | 5.468 |
| Sr (225) | 5.924 | 5.933 | 5.923 | 5.974 | 5.933 | 5.955 | 5.917 | 5.928 |
| Cs (229) | 5.998 | 6.046 | 5.915 | 6.025 | 5.963 | 6.190 | 5.876 | 5.843 |
| Ba (229) | 4.868 | 4.928 | 4.891 | 4.946 | 4.911 | 4.958 | 4.901 | 4.917 |
| V (229) | 2.963 | 2.962 | 2.974 | 2.989 | 2.975 | 2.937 | 2.985 | 3.009 |
| Ni (225) | 3.471 | 3.485 | 3.489 | 3.503 | 3.493 | 3.467 | 3.512 | 3.540 |
| Cu (225) | 3.579 | 3.582 | 3.599 | 3.614 | 3.605 | 3.549 | 3.627 | 3.650 |
| Nb (229) | 3.276 | 3.276 | 3.289 | 3.300 | 3.291 | 3.251 | 3.305 | 3.336 |
| Mo (229) | 3.135 | 3.138 | 3.146 | 3.153 | 3.148 | 3.121 | 3.162 | 3.186 |
| Rh (225) | 3.789 | 3.804 | 3.807 | 3.817 | 3.810 | 3.787 | 3.834 | 3.869 |
| Pd (225) | 3.884 | 3.902 | 3.907 | 3.920 | 3.912 | 3.878 | 3.940 | 3.980 |
| Ag (225) | 4.065 | 4.088 | 4.095 | 4.113 | 4.103 | 4.059 | 4.135 | 4.174 |
| Ta (229) | 3.284 | 3.293 | 3.296 | 3.309 | 3.298 | 3.281 | 3.310 | 3.341 |
| W (229) | 3.159 | 3.166 | 3.169 | 3.177 | 3.171 | 3.156 | 3.183 | 3.207 |
| Ir (225) | 3.840 | 3.851 | 3.855 | 3.861 | 3.858 | 3.835 | 3.881 | 3.913 |
| Pt (225) | 3.927 | 3.941 | 3.947 | 3.954 | 3.951 | 3.919 | 3.978 | 4.018 |
| Au (225) | 4.095 | 4.118 | 4.123 | 4.133 | 4.129 | 4.094 | 4.164 | 4.206 |
| ME | 0.015 | -0.002 | 0.015 | 0.029 | 0.020 | -0.011 | 0.026 | 0.042 |
| MAE | 0.041 | 0.042 | 0.046 | 0.045 | 0.047 | 0.043 | 0.062 | 0.083 |
| MRE | 0.3 | -0.1 | 0.3 | 0.6 | 0.4 | -0.4 | 0.6 | 1.0 |
| MARE | 0.9 | 0.9 | 0.9 | 0.9 | 0.9 | 1.0 | 1.3 | 1.7 |

TABLE S3. Equilibrium lattice constant $a_0$ (in Å) of 44 solids. All results were obtained non-self-consistently using PBE orbitals/density. The space group number is indicated in parenthesis.

| Solid | vdW-DF | vdW-DF2 |
|---|---|---|
| C (227) | 3.600 | 3.608 |
| Si (227) | 5.513 | 5.540 |
| Ge (227) | 5.862 | 5.956 |
| Sn (227) | 6.772 | 6.874 |
| SiC (216) | 4.411 | 4.428 |
| BN (216) | 3.652 | 3.662 |
| BP (216) | 4.591 | 4.609 |
| AlN (216) | 4.430 | 4.440 |
| AlP (216) | 5.553 | 5.573 |
| AlAs (216) | 5.787 | 5.831 |
| GaN (216) | 4.600 | 4.638 |
| GaP (216) | 5.585 | 5.632 |
| GaAs (216) | 5.843 | 5.922 |
| InP (216) | 6.048 | 6.107 |
| InAs (216) | 6.289 | 6.373 |
| InSb (216) | 6.750 | 6.840 |
| LiH (225) | 4.067 | 4.044 |
| LiF (225) | 4.123 | 4.084 |
| LiCl (225) | 5.229 | 5.210 |
| NaF (225) | 4.751 | 4.686 |
| NaCl (225) | 5.750 | 5.686 |
| MgO (225) | 4.286 | 4.287 |
| Li (229) | 3.458 | 3.401 |
| Na (229) | 4.229 | 4.140 |
| Al (225) | 4.083 | 4.074 |
| K (229) | 5.304 | 5.176 |
| Ca (225) | 5.549 | 5.481 |
| Rb (229) | 5.653 | 5.531 |
| Sr (225) | 6.061 | 5.998 |
| Cs (229) | 6.100 | 5.941 |
| Ba (229) | 5.069 | 5.040 |
| V (229) | 3.026 | 3.045 |
| Ni (225) | 3.575 | 3.615 |
| Cu (225) | 3.702 | 3.743 |
| Nb (229) | 3.344 | 3.382 |
| Mo (229) | 3.193 | 3.229 |
| Rh (225) | 3.884 | 3.947 |
| Pd (225) | 4.014 | 4.087 |
| Ag (225) | 4.250 | 4.321 |
| Ta (229) | 3.348 | 3.380 |
| W (229) | 3.212 | 3.245 |
| Ir (225) | 3.919 | 3.982 |
| Pt (225) | 4.032 | 4.113 |
| Au (225) | 4.253 | 4.348 |
| ME | 0.105 | 0.117 |
| MAE | 0.106 | 0.140 |
| MRE | 2.2 | 2.5 |
| MARE | 2.2 | 3.0 |

TABLE S4. Bulk modulus $B_0$ (in GPa) of 44 solids. All results were obtained non-self-consistently using PBE orbitals/density. The space group number is indicated in parenthesis.

| Solid | Expt. | TM | SCAN | PBEsol | PBE | LDA | SCAN+rVV10 | PBEsol+rVV10s | C09-vdW |
|---|---|---|---|---|---|---|---|---|---|
| C (227) | 454.7 | 454.5 | 461.3 | 452.1 | 434.7 | 469.8 | 463.7 | 454.2 | 446.6 |
| Si (227) | 101.3 | 98.1 | 98.8 | 93.1 | 88.3 | 96.0 | 100.0 | 94.7 | 93.6 |
| Ge (227) | 79.4 | 72.4 | 71.1 | 67.5 | 59.2 | 71.9 | 72.9 | 69.1 | 66.5 |
| Sn (227) | 42.8 | 44.2 | 41.6 | 41.7 | 35.9 | 45.1 | 43.2 | 43.4 | 41.7 |
| SiC (216) | 229.1 | 228.2 | 226.0 | 221.9 | 212.9 | 230.4 | 227.6 | 222.6 | 221.0 |
| BN (216) | 410.2 | 390.8 | 397.4 | 388.0 | 373.8 | 404.9 | 399.5 | 389.5 | 385.3 |
| BP (216) | 168.0 | 172.5 | 172.4 | 169.5 | 161.9 | 175.8 | 173.8 | 171.3 | 168.1 |
| AlN (216) | 206.0 | 207.0 | 216.0 | 201.9 | 193.9 | 212.2 | 217.4 | 202.7 | 202.8 |
| AlP (216) | 87.4 | 91.1 | 90.8 | 86.7 | 82.5 | 89.9 | 91.8 | 87.9 | 87.3 |
| AlAs (216) | 75.0 | 76.7 | 76.2 | 72.0 | 67.1 | 75.4 | 77.4 | 73.1 | 72.3 |
| GaN (216) | 213.7 | 191.3 | 200.7 | 189.9 | 173.2 | 203.8 | 203.1 | 192.1 | 189.0 |
| GaP (216) | 89.6 | 88.0 | 87.9 | 85.1 | 77.0 | 90.3 | 89.6 | 87.2 | 84.6 |
| GaAs (216) | 76.7 | 73.2 | 70.5 | 69.0 | 60.8 | 74.0 | 72.4 | 70.8 | 68.4 |
| InP (216) | 72.0 | 68.2 | 69.9 | 66.7 | 59.5 | 71.0 | 71.6 | 68.8 | 66.5 |
| InAs (216) | 58.6 | 57.6 | 58.3 | 55.6 | 48.5 | 60.0 | 60.2 | 57.5 | 55.4 |
| InSb (216) | 46.1 | 44.4 | 44.3 | 42.8 | 36.9 | 46.4 | 45.9 | 44.5 | 42.9 |
| LiH (225) | 40.1 | 40.4 | 36.6 | 37.2 | 36.3 | 40.3 | 36.9 | 37.6 | 35.3 |
| LiF (225) | 76.3 | 78.5 | 75.9 | 72.1 | 66.8 | 86.2 | 77.7 | 74.2 | 71.2 |
| LiCl (225) | 38.7 | 38.3 | 35.6 | 35.0 | 31.7 | 40.6 | 37.2 | 36.6 | 35.3 |
| NaF (225) | 53.1 | 54.7 | 57.5 | 48.3 | 44.6 | 61.2 | 59.3 | 50.4 | 48.8 |
| NaCl (225) | 27.6 | 29.0 | 28.0 | 25.6 | 23.6 | 31.7 | 29.4 | 27.2 | 26.5 |
| MgO (225) | 169.8 | 164.4 | 171.5 | 157.8 | 149.2 | 173.1 | 173.5 | 160.0 | 159.7 |
| Li (229) | 13.1 | 14.5 | 13.1 | 13.6 | 13.7 | 15.1 | 13.1 | 13.5 | 13.1 |
| Na (229) | 7.9 | 8.6 | 7.7 | 7.9 | 7.7 | 9.1 | 7.8 | 8.1 | 7.7 |
| Al (225) | 77.1 | 91.7 | 80.1 | 81.1 | 76.7 | 82.6 | 80.8 | 80.7 | 78.4 |
| K (229) | 3.8 | 4.0 | 3.3 | 3.7 | 3.6 | 4.5 | 3.4 | 3.8 | 3.6 |
| Ca (225) | 15.9 | 18.9 | 17.7 | 17.7 | 17.2 | 19.0 | 17.8 | 18.0 | 17.9 |
| Rb (229) | 3.6 | 3.2 | 2.8 | 2.9 | 2.8 | 3.6 | 2.9 | 3.1 | 3.5 |
| Sr (225) | 12.0 | 12.8 | 11.1 | 12.5 | 11.6 | 14.2 | 11.4 | 12.8 | 12.8 |
| Cs (229) | 2.3 | 2.1 | 1.9 | 2.1 | 2.0 | 2.5 | 2.0 | 2.2 | 2.5 |
| Ba (229) | 10.6 | 9.3 | 8.6 | 9.2 | 8.7 | 10.3 | 8.8 | 9.4 | 9.6 |
| V (229) | 165.8 | 194.5 | 194.6 | 196.1 | 181.5 | 209.1 | 197.3 | 198.1 | 195.9 |
| Ni (225) | 192.5 | 230.6 | 225.2 | 230.0 | 197.2 | 255.6 | 230.4 | 236.4 | 227.1 |
| Cu (225) | 144.3 | 180.6 | 172.6 | 169.4 | 141.9 | 191.1 | 177.4 | 175.1 | 166.8 |
| Nb (229) | 173.2 | 177.2 | 177.8 | 181.0 | 168.5 | 190.4 | 180.1 | 183.2 | 181.5 |
| Mo (229) | 276.2 | 273.3 | 274.5 | 277.9 | 256.7 | 291.2 | 278.2 | 281.7 | 277.3 |
| Rh (225) | 277.1 | 289.8 | 300.6 | 295.4 | 256.8 | 318.3 | 307.9 | 302.8 | 294.2 |
| Pd (225) | 187.2 | 195.7 | 193.4 | 205.1 | 169.0 | 228.1 | 201.2 | 210.4 | 204.7 |
| Ag (225) | 105.7 | 113.3 | 107.4 | 119.0 | 90.6 | 139.2 | 113.5 | 124.1 | 119.5 |
| Ta (229) | 202.7 | 205.5 | 203.9 | 205.0 | 192.6 | 215.7 | 206.6 | 208.1 | 205.8 |
| W (229) | 327.5 | 323.7 | 322.9 | 321.3 | 301.1 | 334.0 | 326.7 | 327.0 | 320.8 |
| Ir (225) | 362.2 | 383.4 | 431.5 | 384.9 | 347.2 | 403.5 | 441.4 | 395.0 | 381.8 |
| Pt (225) | 285.5 | 284.7 | 292.6 | 287.7 | 247.9 | 307.6 | 300.9 | 296.1 | 285.1 |
| Au (225) | 182.0 | 170.3 | 168.1 | 173.4 | 137.5 | 193.6 | 175.5 | 181.0 | 172.3 |
| ME | | 2.4 | 3.5 | 0.7 | -11.2 | 10.1 | 6.0 | 3.2 | 0.1 |
| MAE | | 6.6 | 7.4 | 7.8 | 12.2 | 11.5 | 8.4 | 8.1 | 7.7 |
| MRE | | 2.1 | -0.5 | -1.4 | -9.8 | 8.1 | 1.8 | 0.9 | -0.9 |
| MARE | | 6.2 | 6.5 | 7.0 | 10.9 | 9.4 | 6.6 | 6.3 | 6.5 |

TABLE S5. Bulk modulus $B_0$ (in GPa) of 44 solids. All results were obtained non-self-consistently using PBE orbitals/density. The space group number is indicated in parenthesis.

| Solid | vdW-DF-cx | PBE-D3(BJ) | optB86b-vdW | PBE+rVV10L | rev-vdW-DF2 | revPBE-D3(BJ) | optB88-vdW | rVV10 |
|---|---|---|---|---|---|---|---|---|
| C (227) | 441.7 | 443.3 | 437.9 | 439.3 | 438.5 | 442.1 | 430.9 | 426.3 |
| Si (227) | 92.5 | 88.0 | 90.9 | 90.5 | 90.1 | 88.3 | 88.6 | 87.4 |
| Ge (227) | 65.2 | 61.4 | 62.3 | 62.2 | 60.6 | 61.0 | 58.5 | 55.7 |
| Sn (227) | 40.7 | 38.3 | 38.8 | 38.7 | 37.6 | 38.0 | 36.7 | 36.0 |
| SiC (216) | 218.8 | 221.1 | 216.5 | 215.8 | 215.7 | 225.0 | 213.1 | 206.1 |
| BN (216) | 380.0 | 382.5 | 378.5 | 377.9 | 378.5 | 383.0 | 374.8 | 365.3 |
| BP (216) | 165.7 | 169.8 | 164.1 | 164.8 | 164.0 | 174.3 | 160.9 | 159.7 |
| AlN (216) | 199.9 | 201.7 | 199.4 | 196.4 | 198.1 | 204.0 | 198.1 | 190.9 |
| AlP (216) | 86.1 | 88.2 | 85.1 | 84.5 | 84.3 | 91.5 | 83.8 | 82.1 |
| AlAs (216) | 71.2 | 72.6 | 69.9 | 69.3 | 69.0 | 75.7 | 68.2 | 65.7 |
| GaN (216) | 185.8 | 181.4 | 181.2 | 178.1 | 179.0 | 181.8 | 176.1 | 166.8 |
| GaP (216) | 83.0 | 83.6 | 80.5 | 80.1 | 79.1 | 86.6 | 77.1 | 75.6 |
| GaAs (216) | 66.9 | 67.0 | 64.3 | 64.0 | 62.8 | 69.7 | 61.0 | 58.8 |
| InP (216) | 65.0 | 64.8 | 62.9 | 62.6 | 61.5 | 66.1 | 60.0 | 59.3 |
| InAs (216) | 54.1 | 53.6 | 51.9 | 51.7 | 50.5 | 55.0 | 49.3 | 48.2 |
| InSb (216) | 41.6 | 41.4 | 39.9 | 39.7 | 38.8 | 42.6 | 37.9 | 37.5 |
| LiH (225) | 32.9 | 40.6 | 35.3 | 36.9 | 35.6 | 41.7 | 35.8 | 36.6 |
| LiF (225) | 66.0 | 73.4 | 70.1 | 69.8 | 69.6 | 70.6 | 71.8 | 74.1 |
| LiCl (225) | 34.1 | 36.8 | 34.5 | 34.2 | 34.0 | 37.8 | 34.7 | 36.4 |
| NaF (225) | 43.0 | 49.6 | 48.5 | 47.4 | 48.0 | 45.4 | 50.6 | 52.1 |
| NaCl (225) | 23.9 | 27.2 | 26.3 | 25.8 | 25.9 | 25.9 | 27.1 | 28.5 |
| MgO (225) | 153.9 | 158.4 | 156.4 | 152.6 | 155.2 | 158.6 | 156.8 | 151.6 |
| Li (229) | 12.9 | 15.5 | 13.1 | 13.9 | 13.6 | 15.5 | 13.8 | 14.2 |
| Na (229) | 7.2 | 8.8 | 7.8 | 7.9 | 7.8 | 8.6 | 8.0 | 8.4 |
| Al (225) | 77.5 | 85.3 | 75.2 | 77.9 | 73.0 | 92.1 | 68.7 | 77.5 |
| K (229) | 3.4 | 4.1 | 3.7 | 3.8 | 3.7 | 3.9 | 3.6 | 4.2 |
| Ca (225) | 17.3 | 18.1 | 17.7 | 17.6 | 17.5 | 17.7 | 17.7 | 18.3 |
| Rb (229) | 3.3 | 3.1 | 3.5 | 3.0 | 3.5 | 2.8 | 3.6 | 3.4 |
| Sr (225) | 12.2 | 12.4 | 12.5 | 12.1 | 12.4 | 11.9 | 12.6 | 13.0 |
| Cs (229) | 2.1 | 2.1 | 2.4 | 2.1 | 2.4 | 1.9 | 2.6 | 2.5 |
| Ba (229) | 9.2 | 9.1 | 9.4 | 9.1 | 9.3 | 8.5 | 9.7 | 10.1 |
| V (229) | 193.1 | 195.9 | 189.2 | 185.9 | 188.0 | 202.9 | 184.3 | 183.0 |
| Ni (225) | 222.0 | 208.2 | 211.6 | 206.4 | 208.5 | 211.9 | 198.6 | 190.9 |
| Cu (225) | 162.0 | 163.5 | 153.6 | 150.3 | 150.4 | 176.0 | 142.5 | 140.2 |
| Nb (229) | 179.6 | 178.8 | 175.7 | 172.8 | 174.6 | 183.5 | 171.0 | 169.2 |
| Mo (229) | 274.7 | 271.6 | 267.2 | 263.7 | 265.4 | 279.1 | 257.0 | 250.5 |
| Rh (225) | 289.5 | 276.8 | 275.7 | 269.8 | 272.3 | 285.8 | 257.1 | 241.3 |
| Pd (225) | 199.9 | 189.2 | 187.7 | 181.9 | 184.3 | 197.7 | 173.3 | 162.4 |
| Ag (225) | 115.1 | 107.7 | 106.2 | 101.5 | 103.1 | 113.0 | 96.8 | 93.8 |
| Ta (229) | 204.1 | 202.4 | 200.1 | 197.0 | 199.0 | 205.0 | 195.5 | 193.0 |
| W (229) | 318.1 | 315.1 | 310.9 | 307.9 | 308.8 | 320.8 | 300.0 | 294.2 |
| Ir (225) | 377.9 | 367.1 | 363.0 | 360.2 | 359.3 | 378.2 | 340.5 | 321.1 |
| Pt (225) | 280.7 | 270.1 | 265.6 | 262.4 | 261.9 | 282.3 | 244.6 | 228.1 |
| Au (225) | 167.8 | 156.6 | 155.0 | 151.4 | 151.5 | 163.5 | 139.3 | 133.0 |
| ME | -2.3 | -3.1 | -5.5 | -6.9 | -6.8 | -0.4 | -10.3 | -13.4 |
| MAE | 8.4 | 7.5 | 8.2 | 8.9 | 9.0 | 8.5 | 11.5 | 14.5 |
| MRE | -4.2 | -2.1 | -4.6 | -5.9 | -5.7 | -1.4 | -6.8 | -7.5 |
| MARE | 8.0 | 7.4 | 7.0 | 7.8 | 7.8 | 8.6 | 9.2 | 10.7 |

TABLE S6. Bulk modulus $B_0$ (in GPa) of 44 solids. All results were obtained non-self-consistently using PBE orbitals/density. The space group number is indicated in parenthesis.

| Solid | vdW-DF | vdW-DF2 |
|---|---|---|
| C (227) | 409.4 | 400.5 |
| Si (227) | 82.7 | 78.7 |
| Ge (227) | 50.0 | 42.4 |
| Sn (227) | 30.5 | 27.0 |
| SiC (216) | 201.6 | 192.3 |
| BN (216) | 356.6 | 347.5 |
| BP (216) | 151.3 | 147.0 |
| AlN (216) | 187.2 | 182.5 |
| AlP (216) | 78.2 | 75.2 |
| AlAs (216) | 62.4 | 58.0 |
| GaN (216) | 157.6 | 146.1 |
| GaP (216) | 68.2 | 62.7 |
| GaAs (216) | 52.4 | 46.1 |
| InP (216) | 52.1 | 47.6 |
| InAs (216) | 41.6 | 37.3 |
| InSb (216) | 31.4 | 28.5 |
| LiH (225) | 33.6 | 34.0 |
| LiF (225) | 63.2 | 69.6 |
| LiCl (225) | 30.5 | 32.9 |
| NaF (225) | 44.0 | 50.5 |
| NaCl (225) | 23.4 | 26.1 |
| MgO (225) | 143.7 | 144.6 |
| Li (229) | 13.7 | 14.6 |
| Na (229) | 7.7 | 8.3 |
| Al (225) | 64.5 | 61.4 |
| K (229) | 3.7 | 3.9 |
| Ca (225) | 16.7 | 17.5 |
| Rb (229) | 3.5 | 3.7 |
| Sr (225) | 11.2 | 12.3 |
| Cs (229) | 2.2 | 2.6 |
| Ba (229) | 8.7 | 9.7 |
| V (229) | 168.2 | 165.8 |
| Ni (225) | 165.8 | 152.5 |
| Cu (225) | 114.6 | 104.8 |
| Nb (229) | 157.7 | 154.1 |
| Mo (229) | 236.2 | 222.6 |
| Rh (225) | 220.3 | 191.0 |
| Pd (225) | 138.1 | 121.0 |
| Ag (225) | 68.3 | 64.2 |
| Ta (229) | 182.1 | 177.5 |
| W (229) | 280.6 | 265.2 |
| Ir (225) | 306.7 | 263.5 |
| Pt (225) | 207.2 | 172.2 |
| Au (225) | 103.8 | 87.9 |
| ME | -23.0 | -29.4 |
| MAE | 23.2 | 29.5 |
| MRE | -16.6 | -18.2 |
| MARE | 17.1 | 20.4 |

TABLE S7. Cohesive energy $E_{coh}$ (in eV/atom) of 44 solids. All results were obtained non-self-consistently using PBE orbitals/density. The space group number is indicated in parenthesis.

| Solid | Expt. | TM | SCAN | PBEsol | PBE | LDA | SCAN+rVV10 | PBEsol+rVV10s | C09-vdW |
|---|---|---|---|---|---|---|---|---|---|
| C (227) | 7.55 | 7.64 | 7.56 | 8.26 | 7.71 | 8.94 | 7.65 | 8.37 | 7.99 |
| Si (227) | 4.68 | 4.76 | 4.73 | 4.94 | 4.57 | 5.33 | 4.84 | 5.07 | 4.90 |
| Ge (227) | 3.89 | 4.03 | 3.96 | 4.15 | 3.73 | 4.63 | 4.09 | 4.29 | 4.12 |
| Sn (227) | 3.16 | 3.46 | 3.37 | 3.55 | 3.17 | 4.00 | 3.51 | 3.70 | 3.56 |
| SiC (216) | 6.48 | 6.52 | 6.49 | 6.87 | 6.40 | 7.41 | 6.59 | 6.98 | 6.73 |
| BN (216) | 6.76 | 6.96 | 6.88 | 7.40 | 6.93 | 8.04 | 6.96 | 7.49 | 7.18 |
| BP (216) | 5.14 | 5.40 | 5.34 | 5.73 | 5.29 | 6.24 | 5.44 | 5.85 | 5.61 |
| AlN (216) | 5.85 | 5.89 | 5.81 | 6.06 | 5.70 | 6.59 | 5.90 | 6.14 | 5.96 |
| AlP (216) | 4.32 | 4.31 | 4.25 | 4.42 | 4.08 | 4.81 | 4.34 | 4.54 | 4.40 |
| AlAs (216) | 3.82 | 3.94 | 3.88 | 4.04 | 3.68 | 4.47 | 3.98 | 4.15 | 4.03 |
| GaN (216) | 4.55 | 4.67 | 4.45 | 4.84 | 4.40 | 5.40 | 4.56 | 4.95 | 4.72 |
| GaP (216) | 3.61 | 3.77 | 3.64 | 3.89 | 3.49 | 4.34 | 3.76 | 4.03 | 3.85 |
| GaAs (216) | 3.34 | 3.47 | 3.33 | 3.55 | 3.15 | 4.04 | 3.45 | 3.68 | 3.53 |
| InP (216) | 3.47 | 3.42 | 3.28 | 3.53 | 3.14 | 3.96 | 3.40 | 3.67 | 3.51 |
| InAs (216) | 3.08 | 3.19 | 3.05 | 3.27 | 2.89 | 3.74 | 3.18 | 3.41 | 3.27 |
| InSb (216) | 2.81 | 2.91 | 2.80 | 3.00 | 2.64 | 3.46 | 2.94 | 3.15 | 3.02 |
| LiH (225) | 2.49 | 2.45 | 2.45 | 2.44 | 2.35 | 2.67 | 2.47 | 2.47 | 2.46 |
| LiF (225) | 4.46 | 4.36 | 4.42 | 4.48 | 4.33 | 4.92 | 4.46 | 4.53 | 4.46 |
| LiCl (225) | 3.59 | 3.47 | 3.52 | 3.52 | 3.37 | 3.84 | 3.58 | 3.59 | 3.56 |
| NaF (225) | 3.97 | 3.88 | 3.93 | 3.97 | 3.84 | 4.37 | 3.97 | 4.02 | 3.97 |
| NaCl (225) | 3.34 | 3.23 | 3.28 | 3.23 | 3.10 | 3.50 | 3.34 | 3.30 | 3.27 |
| MgO (225) | 5.20 | 5.20 | 5.25 | 5.32 | 4.99 | 5.84 | 5.33 | 5.40 | 5.29 |
| Li (229) | 1.67 | 1.68 | 1.58 | 1.68 | 1.61 | 1.80 | 1.61 | 1.73 | 1.58 |
| Na (229) | 1.12 | 1.20 | 1.07 | 1.15 | 1.08 | 1.24 | 1.11 | 1.21 | 1.05 |
| Al (225) | 3.43 | 3.86 | 3.60 | 3.81 | 3.44 | 4.01 | 3.70 | 3.99 | 3.69 |
| K (229) | 0.94 | 1.00 | 0.85 | 0.93 | 0.87 | 1.01 | 0.90 | 1.01 | 0.89 |
| Ca (225) | 1.87 | 2.29 | 2.08 | 2.11 | 1.91 | 2.20 | 2.18 | 2.24 | 2.11 |
| Rb (229) | 0.86 | 0.92 | 0.74 | 0.84 | 0.78 | 0.92 | 0.80 | 0.92 | 0.81 |
| Sr (225) | 1.73 | 2.05 | 1.80 | 1.81 | 1.61 | 1.88 | 1.90 | 1.95 | 1.85 |
| Cs (229) | 0.81 | 0.85 | 0.67 | 0.78 | 0.72 | 0.88 | 0.74 | 0.87 | 0.78 |
| Ba (229) | 1.91 | 2.34 | 2.06 | 2.13 | 1.89 | 2.24 | 2.20 | 2.29 | 2.22 |
| V (229) | 5.35 | 5.86 | 4.69 | 6.00 | 5.37 | 6.76 | 4.87 | 6.23 | 5.89 |
| Ni (225) | 4.48 | 5.45 | 4.61 | 5.50 | 4.76 | 6.21 | 4.78 | 5.72 | 5.38 |
| Cu (225) | 3.51 | 4.45 | 3.98 | 4.07 | 3.52 | 4.55 | 4.13 | 4.27 | 3.99 |
| Nb (229) | 7.60 | 7.56 | 6.62 | 7.71 | 6.98 | 8.57 | 6.85 | 8.00 | 7.73 |
| Mo (229) | 6.86 | 6.96 | 5.87 | 7.10 | 6.28 | 8.10 | 6.12 | 7.41 | 7.16 |
| Rh (225) | 5.78 | 6.41 | 5.48 | 6.69 | 5.74 | 7.62 | 5.73 | 6.98 | 6.68 |
| Pd (225) | 3.93 | 4.58 | 4.25 | 4.44 | 3.71 | 5.07 | 4.49 | 4.71 | 4.50 |
| Ag (225) | 2.96 | 3.28 | 2.89 | 3.09 | 2.53 | 3.66 | 3.10 | 3.33 | 3.16 |
| Ta (229) | 8.13 | 9.12 | 8.55 | 9.03 | 8.22 | 9.66 | 8.81 | 9.36 | 8.98 |
| W (229) | 8.94 | 9.30 | 8.75 | 9.13 | 8.34 | 10.15 | 9.03 | 9.48 | 9.16 |
| Ir (225) | 6.99 | 8.27 | 7.74 | 8.39 | 7.35 | 9.33 | 8.05 | 8.73 | 8.39 |
| Pt (225) | 5.87 | 6.53 | 6.18 | 6.43 | 5.55 | 7.15 | 6.47 | 6.74 | 6.51 |
| Au (225) | 3.83 | 3.91 | 3.56 | 3.72 | 3.03 | 4.33 | 3.82 | 4.00 | 3.83 |
| ME | | 0.24 | -0.02 | 0.29 | -0.13 | 0.77 | 0.11 | 0.45 | 0.27 |
| MAE | | 0.27 | 0.19 | 0.31 | 0.19 | 0.77 | 0.22 | 0.45 | 0.28 |
| MRE | | 6.4 | -0.7 | 6.1 | -3.9 | 17.2 | 2.9 | 10.5 | 5.4 |
| MARE | | 7.0 | 4.9 | 6.9 | 5.0 | 17.2 | 5.4 | 10.6 | 6.7 |

TABLE S8. Cohesive energy $E_{\mathrm{coh}}$ (in eV/atom) of 44 solids. All results were obtained non-self-consistently using PBE orbitals/density. The space group number is indicated in parenthesis.

| Solid | vdW-DF-cx | PBE-D3(BJ) | optB86b-vdW | PBE+rVV10L | rev-vdW-DF2 | revPBE-D3(BJ) | optB88-vdW | rVV10 |
|---|---|---|---|---|---|---|---|---|
| C (227) | 7.79 | 7.89 | 7.78 | 7.89 | 7.77 | 7.64 | 7.59 | 7.64 |
| Si (227) | 4.80 | 4.86 | 4.74 | 4.75 | 4.67 | 4.87 | 4.60 | 4.60 |
| Ge (227) | 4.00 | 4.00 | 3.95 | 3.95 | 3.87 | 3.92 | 3.85 | 3.91 |
| Sn (227) | 3.44 | 3.45 | 3.42 | 3.41 | 3.33 | 3.35 | 3.34 | 3.48 |
| SiC (216) | 6.58 | 6.68 | 6.55 | 6.59 | 6.50 | 6.60 | 6.40 | 6.37 |
| BN (216) | 6.99 | 7.12 | 7.01 | 7.10 | 7.01 | 6.91 | 6.92 | 6.96 |
| BP (216) | 5.46 | 5.60 | 5.43 | 5.48 | 5.39 | 5.57 | 5.28 | 5.31 |
| AlN (216) | 5.81 | 5.94 | 5.84 | 5.86 | 5.80 | 5.83 | 5.80 | 5.82 |
| AlP (216) | 4.30 | 4.37 | 4.27 | 4.26 | 4.20 | 4.38 | 4.17 | 4.15 |
| AlAs (216) | 3.92 | 3.98 | 3.89 | 3.87 | 3.82 | 3.96 | 3.80 | 3.83 |
| GaN (216) | 4.55 | 4.63 | 4.56 | 4.60 | 4.51 | 4.47 | 4.48 | 4.53 |
| GaP (216) | 3.74 | 3.78 | 3.69 | 3.69 | 3.61 | 3.74 | 3.58 | 3.59 |
| GaAs (216) | 3.41 | 3.45 | 3.37 | 3.36 | 3.29 | 3.39 | 3.28 | 3.36 |
| InP (216) | 3.40 | 3.43 | 3.36 | 3.36 | 3.28 | 3.37 | 3.27 | 3.31 |
| InAs (216) | 3.15 | 3.18 | 3.13 | 3.12 | 3.05 | 3.10 | 3.05 | 3.16 |
| InSb (216) | 2.90 | 2.94 | 2.88 | 2.87 | 2.80 | 2.86 | 2.82 | 2.96 |
| LiH (225) | 2.44 | 2.51 | 2.46 | 2.40 | 2.46 | 2.58 | 2.47 | 2.44 |
| LiF (225) | 4.38 | 4.49 | 4.45 | 4.40 | 4.44 | 4.42 | 4.48 | 4.46 |
| LiCl (225) | 3.50 | 3.58 | 3.53 | 3.47 | 3.49 | 3.60 | 3.53 | 3.53 |
| NaF (225) | 3.91 | 4.00 | 3.96 | 3.92 | 3.94 | 3.93 | 3.99 | 3.96 |
| NaCl (225) | 3.24 | 3.31 | 3.25 | 3.21 | 3.20 | 3.32 | 3.26 | 3.24 |
| MgO (225) | 5.17 | 5.26 | 5.19 | 5.13 | 5.13 | 5.20 | 5.18 | 5.14 |
| Li (229) | 1.58 | 1.78 | 1.56 | 1.66 | 1.55 | 1.84 | 1.50 | 1.64 |
| Na (229) | 1.06 | 1.23 | 1.03 | 1.15 | 1.00 | 1.26 | 0.97 | 1.11 |
| Al (225) | 3.61 | 3.76 | 3.49 | 3.63 | 3.38 | 3.84 | 3.22 | 3.36 |
| K (229) | 0.89 | 0.98 | 0.88 | 0.96 | 0.83 | 0.97 | 0.83 | 0.95 |
| Ca (225) | 2.05 | 2.13 | 2.00 | 2.07 | 1.88 | 2.15 | 1.88 | 2.00 |
| Rb (229) | 0.80 | 0.88 | 0.80 | 0.88 | 0.75 | 0.84 | 0.76 | 0.88 |
| Sr (225) | 1.79 | 1.81 | 1.74 | 1.80 | 1.60 | 1.78 | 1.62 | 1.73 |
| Cs (229) | 0.75 | 0.80 | 0.77 | 0.84 | 0.72 | 0.74 | 0.74 | 0.87 |
| Ba (229) | 2.15 | 2.09 | 2.09 | 2.12 | 1.95 | 2.01 | 1.99 | 2.10 |
| V (229) | 5.71 | 5.99 | 5.64 | 5.69 | 5.60 | 6.11 | 5.39 | 5.67 |
| Ni (225) | 5.19 | 5.18 | 5.07 | 5.06 | 4.96 | 5.12 | 4.80 | 4.88 |
| Cu (225) | 3.83 | 4.03 | 3.75 | 3.79 | 3.64 | 4.17 | 3.56 | 3.72 |
| Nb (229) | 7.55 | 7.65 | 7.44 | 7.40 | 7.38 | 7.74 | 7.15 | 7.29 |
| Mo (229) | 6.96 | 6.92 | 6.84 | 6.74 | 6.79 | 6.96 | 6.53 | 6.60 |
| Rh (225) | 6.46 | 6.30 | 6.28 | 6.19 | 6.18 | 6.27 | 5.95 | 5.90 |
| Pd (225) | 4.30 | 4.29 | 4.19 | 4.12 | 4.07 | 4.36 | 3.99 | 4.12 |
| Ag (225) | 2.99 | 3.05 | 2.93 | 2.88 | 2.81 | 3.12 | 2.79 | 2.92 |
| Ta (229) | 8.80 | 8.82 | 8.59 | 8.67 | 8.44 | 8.82 | 8.22 | 8.43 |
| W (229) | 8.93 | 8.96 | 8.83 | 8.84 | 8.80 | 8.87 | 8.51 | 8.88 |
| Ir (225) | 8.16 | 7.97 | 7.93 | 7.89 | 7.82 | 7.96 | 7.52 | 7.52 |
| Pt (225) | 6.31 | 6.20 | 6.13 | 6.05 | 5.99 | 6.31 | 5.81 | 5.86 |
| Au (225) | 3.64 | 3.59 | 3.54 | 3.48 | 3.41 | 3.65 | 3.34 | 3.47 |
| ME | 0.14 | 0.20 | 0.09 | 0.10 | 0.02 | 0.18 | -0.04 | 0.04 |
| MAE | 0.19 | 0.21 | 0.16 | 0.17 | 0.14 | 0.21 | 0.13 | 0.13 |
| MRE | 2.5 | 4.8 | 1.4 | 2.4 | -0.9 | 4.2 | -2.0 | 1.1 |
| MARE | 4.8 | 5.2 | 4.0 | 4.1 | 4.0 | 5.2 | 3.8 | 3.2 |

TABLE S9. Cohesive energy $E_{coh}$ (in eV/atom) of 44 solids. All results were obtained non-self-consistently using PBE orbitals/density. The space group number is indicated in parenthesis.

| Solid | vdW-DF | vdW-DF2 |
|---|---|---|
| C (227) | 6.99 | 6.86 |
| Si (227) | 4.19 | 4.00 |
| Ge (227) | 3.37 | 3.33 |
| Sn (227) | 2.91 | 2.95 |
| SiC (216) | 5.88 | 5.70 |
| BN (216) | 6.38 | 6.36 |
| BP (216) | 4.80 | 4.66 |
| AlN (216) | 5.36 | 5.38 |
| AlP (216) | 3.79 | 3.64 |
| AlAs (216) | 3.39 | 3.33 |
| GaN (216) | 3.98 | 3.95 |
| GaP (216) | 3.13 | 3.01 |
| GaAs (216) | 2.82 | 2.81 |
| InP (216) | 2.85 | 2.76 |
| InAs (216) | 2.62 | 2.66 |
| InSb (216) | 2.39 | 2.46 |
| LiH (225) | 2.41 | 2.46 |
| LiF (225) | 4.31 | 4.45 |
| LiCl (225) | 3.37 | 3.42 |
| NaF (225) | 3.85 | 3.94 |
| NaCl (225) | 3.14 | 3.14 |
| MgO (225) | 4.78 | 4.83 |
| Li (229) | 1.46 | 1.42 |
| Na (229) | 0.93 | 0.85 |
| Al (225) | 2.83 | 2.44 |
| K (229) | 0.79 | 0.71 |
| Ca (225) | 1.63 | 1.40 |
| Rb (229) | 0.71 | 0.64 |
| Sr (225) | 1.36 | 1.12 |
| Cs (229) | 0.67 | 0.62 |
| Ba (229) | 1.68 | 1.48 |
| V (229) | 4.78 | 4.77 |
| Ni (225) | 4.02 | 3.83 |
| Cu (225) | 2.96 | 2.85 |
| Nb (229) | 6.42 | 6.30 |
| Mo (229) | 5.72 | 5.59 |
| Rh (225) | 4.96 | 4.67 |
| Pd (225) | 3.18 | 3.14 |
| Ag (225) | 2.17 | 2.18 |
| Ta (229) | 7.31 | 6.95 |
| W (229) | 7.68 | 7.73 |
| Ir (225) | 6.41 | 6.02 |
| Pt (225) | 4.86 | 4.60 |
| Au (225) | 2.59 | 2.54 |
| ME | -0.51 | -0.59 |
| MAE | 0.51 | 0.59 |
| MRE | -12.8 | -15.6 |
| MARE | 12.8 | 15.6 |

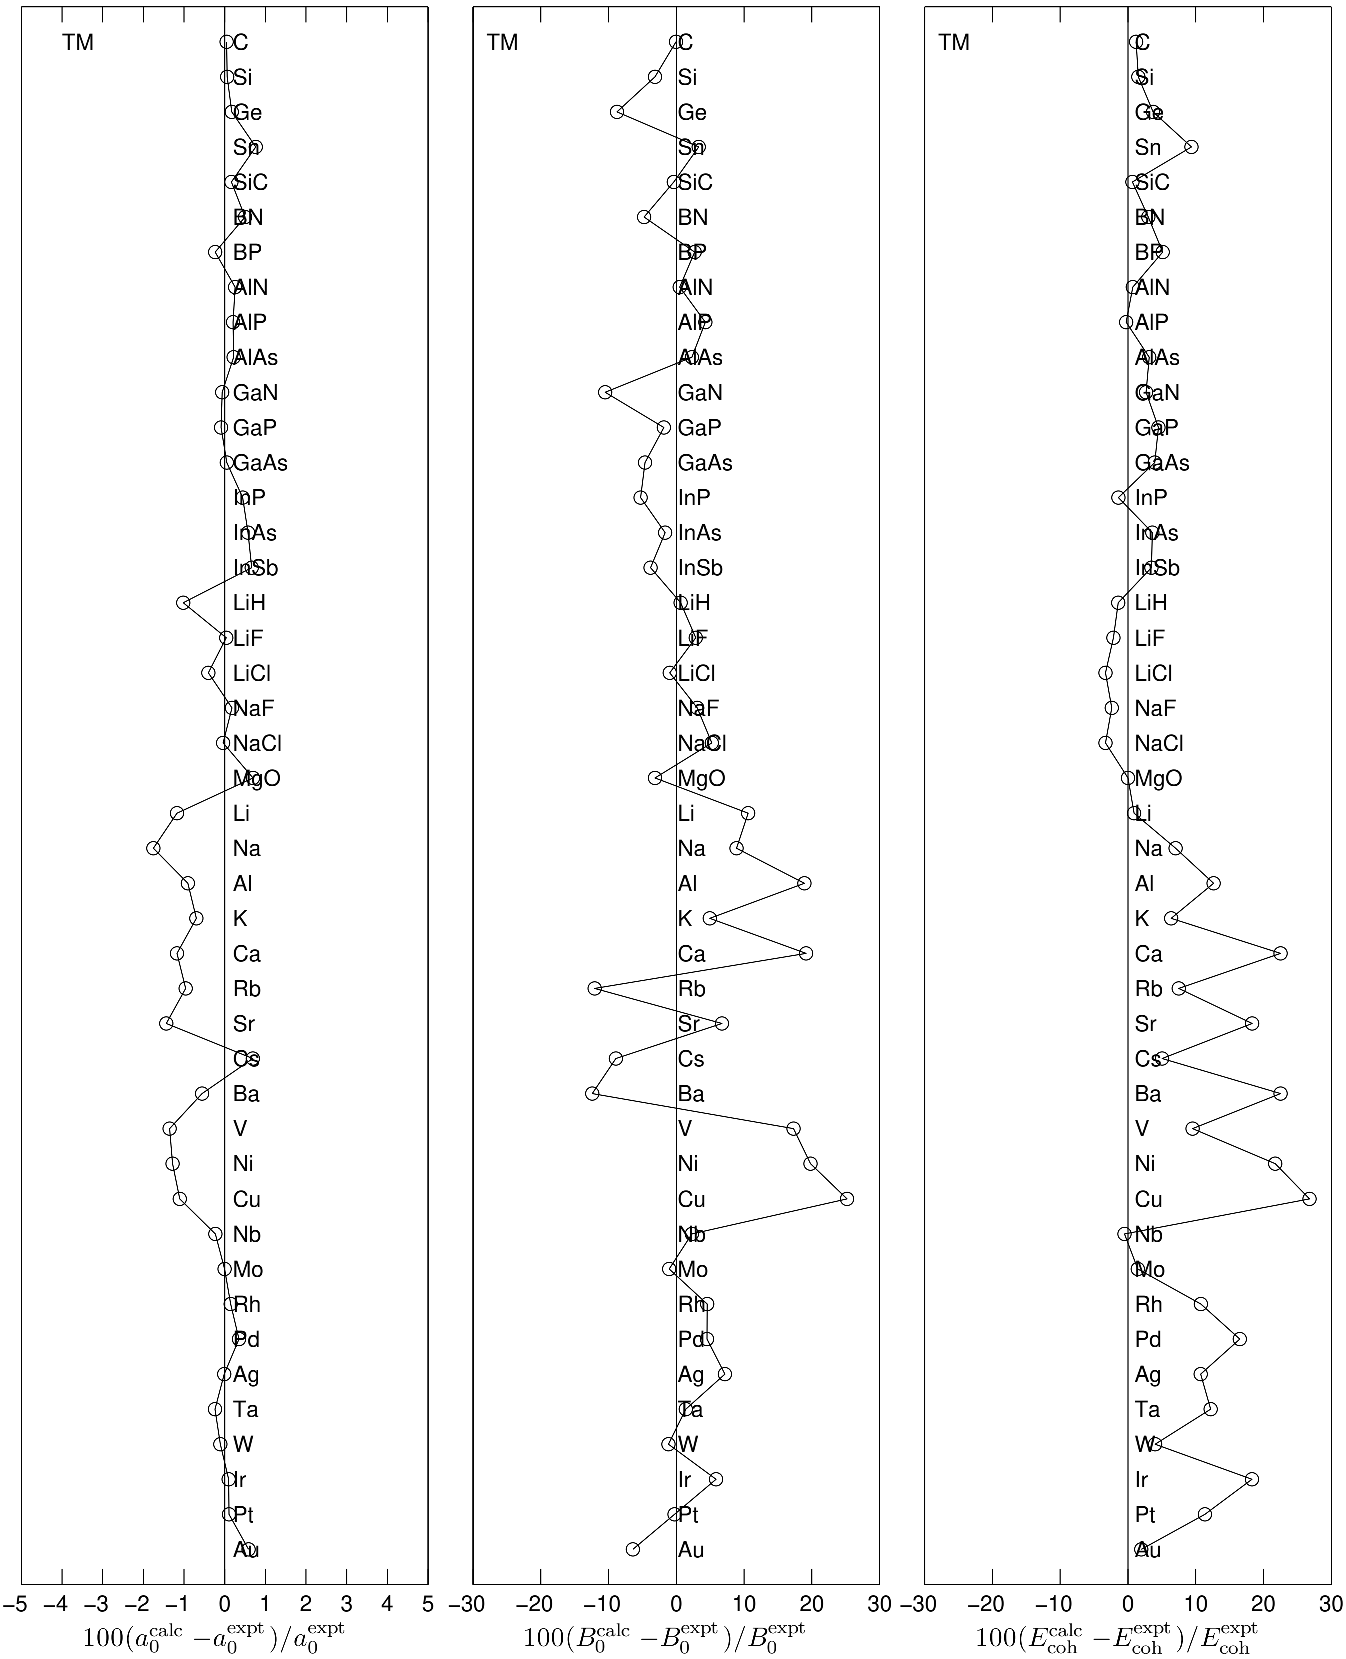


FIG. S1. Relative error (in %) in the calculated lattice constants $a_0$ (left), bulk modulus $B_0$ (middle), and cohesive energy $E_{\rm coh}$ (right) with respect to the experimental values.

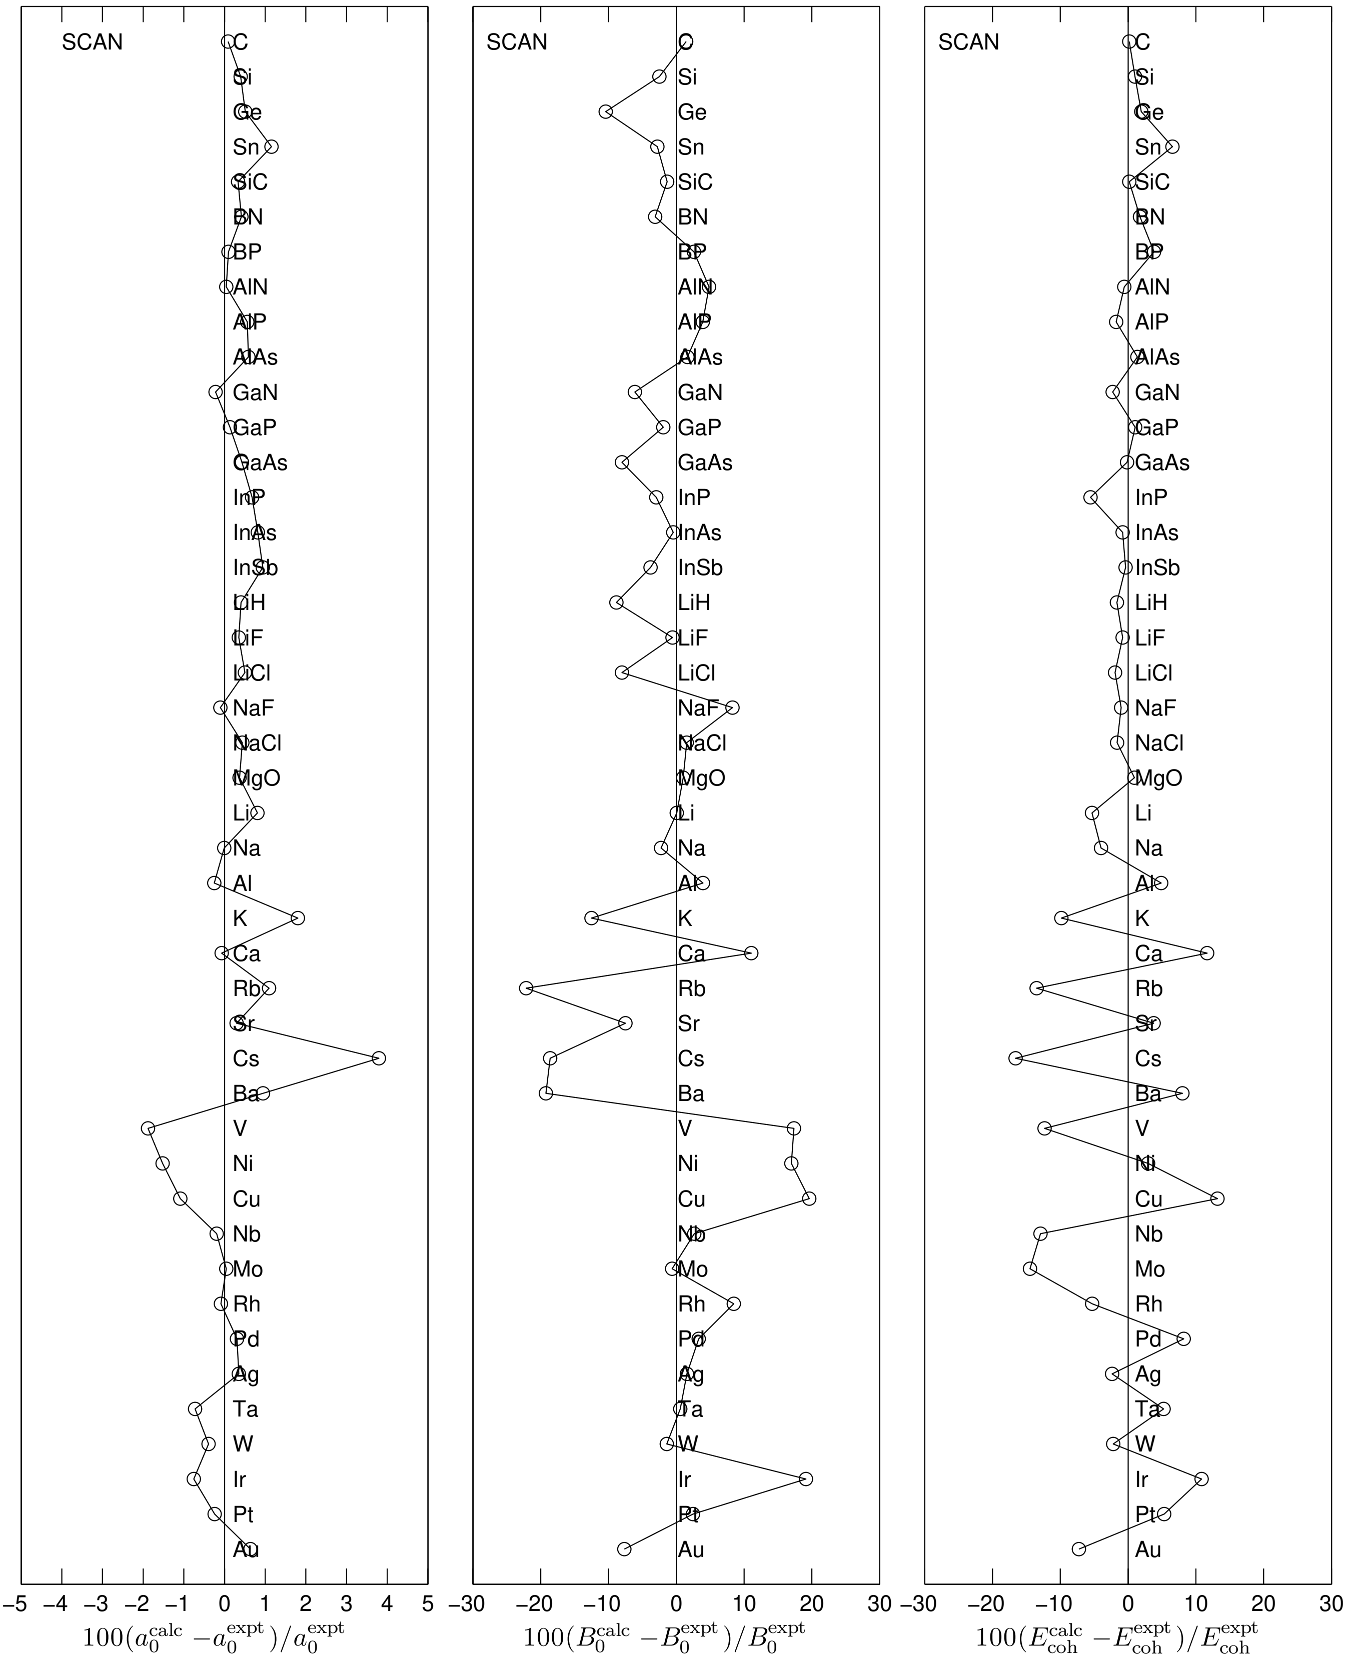


FIG. S2. Relative error (in %) in the calculated lattice constants $a_0$ (left), bulk modulus $B_0$ (middle), and cohesive energy $E_{\mathrm{coh}}$ (right) with respect to the experimental values.

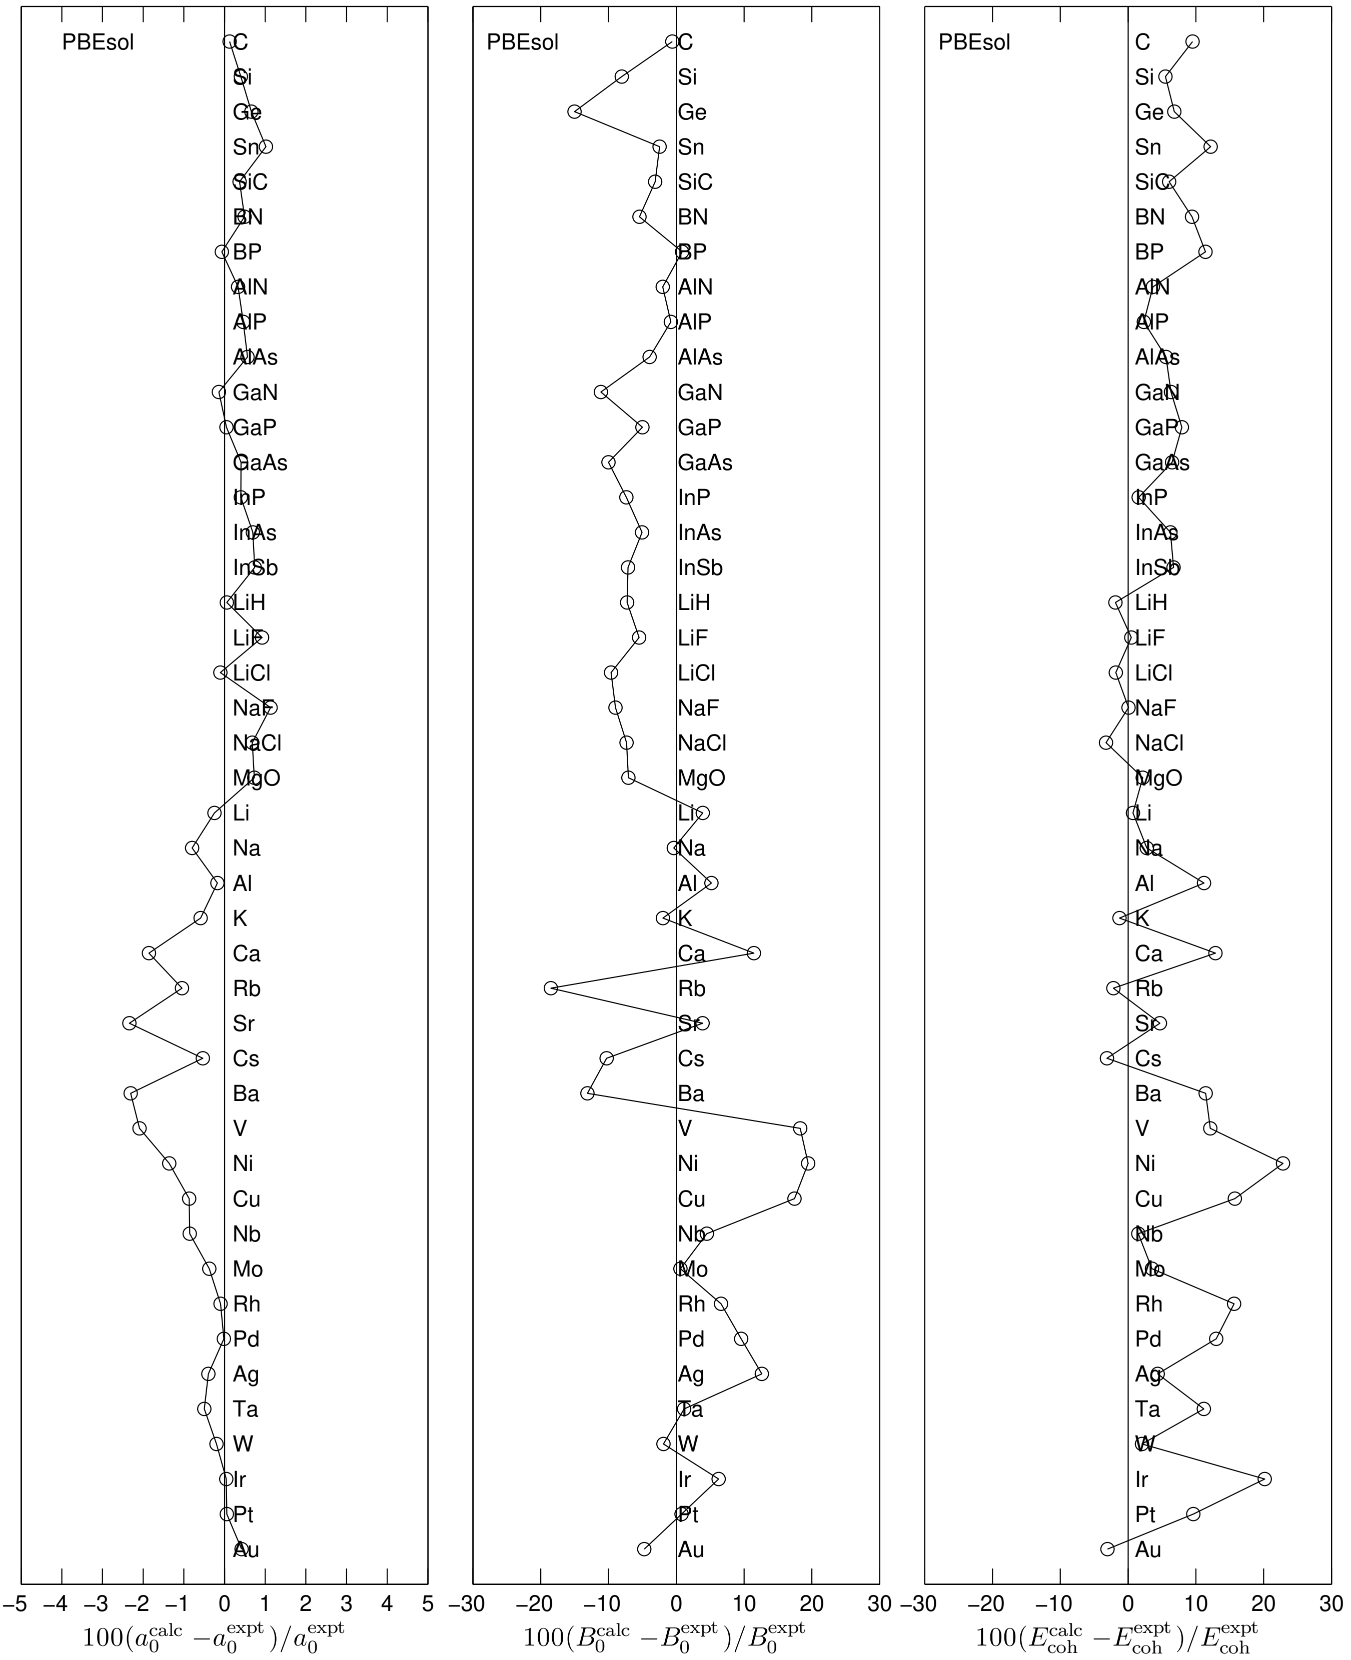


FIG. S3. Relative error (in %) in the calculated lattice constants $a_0$ (left), bulk modulus $B_0$ (middle), and cohesive energy $E_{coh}$ (right) with respect to the experimental values.

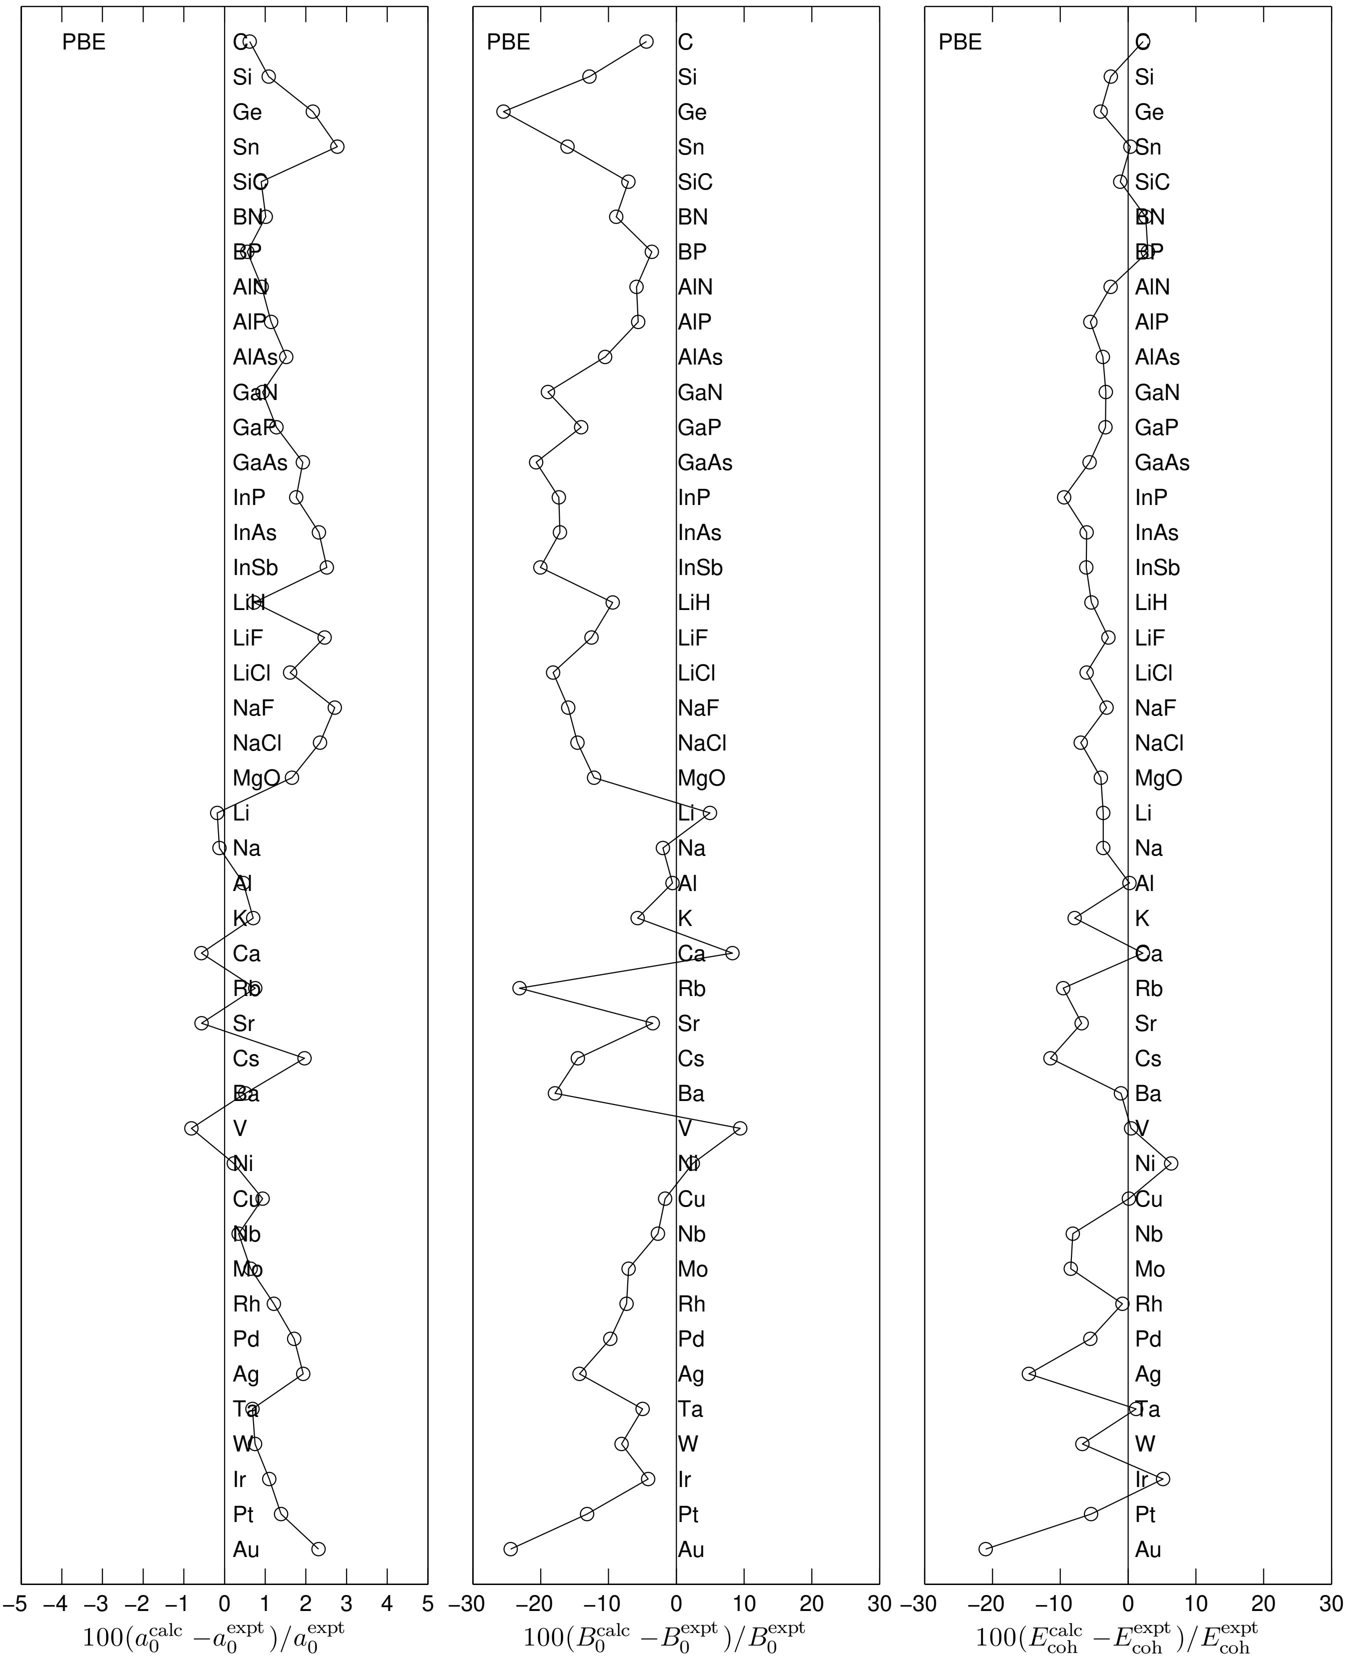


FIG. S4. Relative error (in %) in the calculated lattice constants $a_0$ (left), bulk modulus $B_0$ (middle), and cohesive energy $E_{coh}$ (right) with respect to the experimental values.

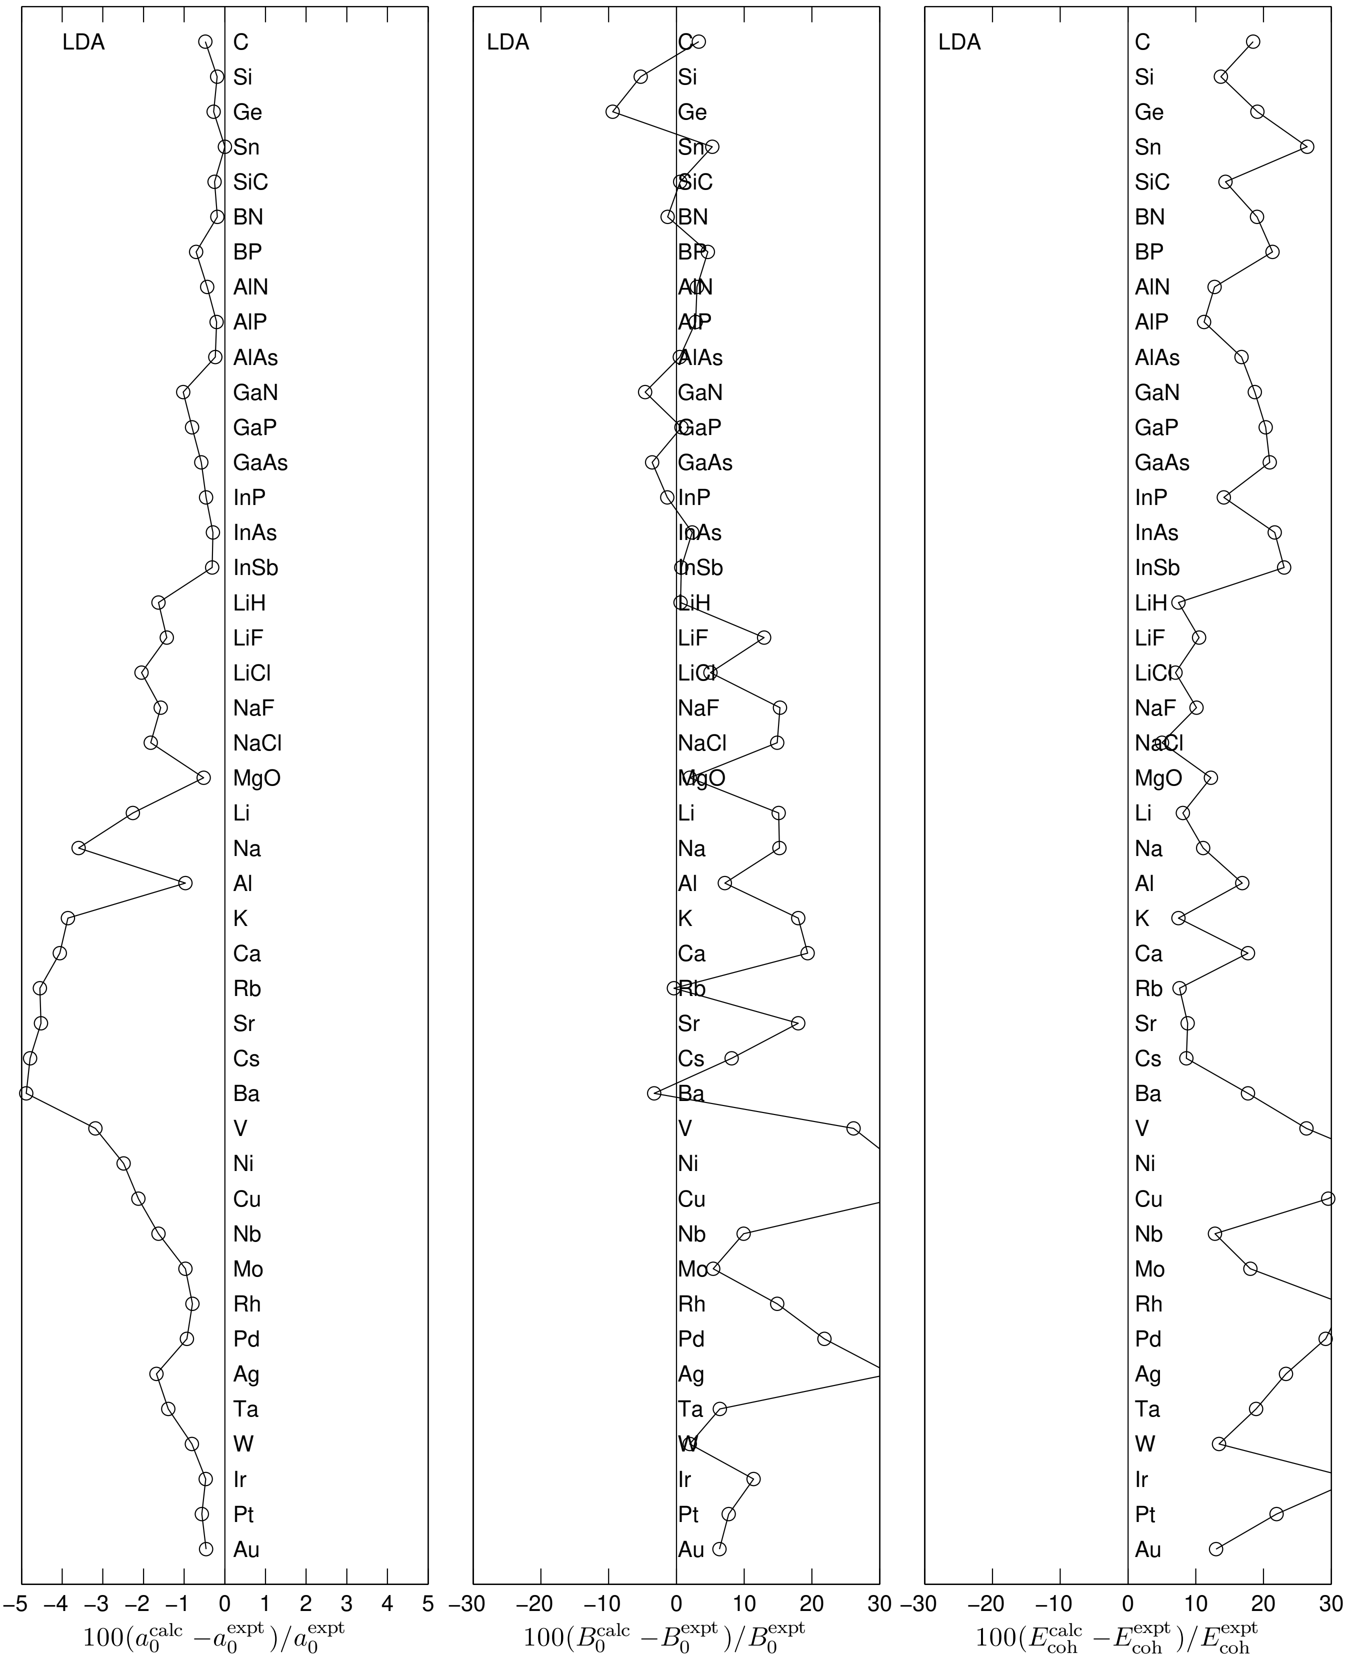


FIG. S5. Relative error (in %) in the calculated lattice constants $a_0$ (left), bulk modulus $B_0$ (middle), and cohesive energy $E_{coh}$ (right) with respect to the experimental values.

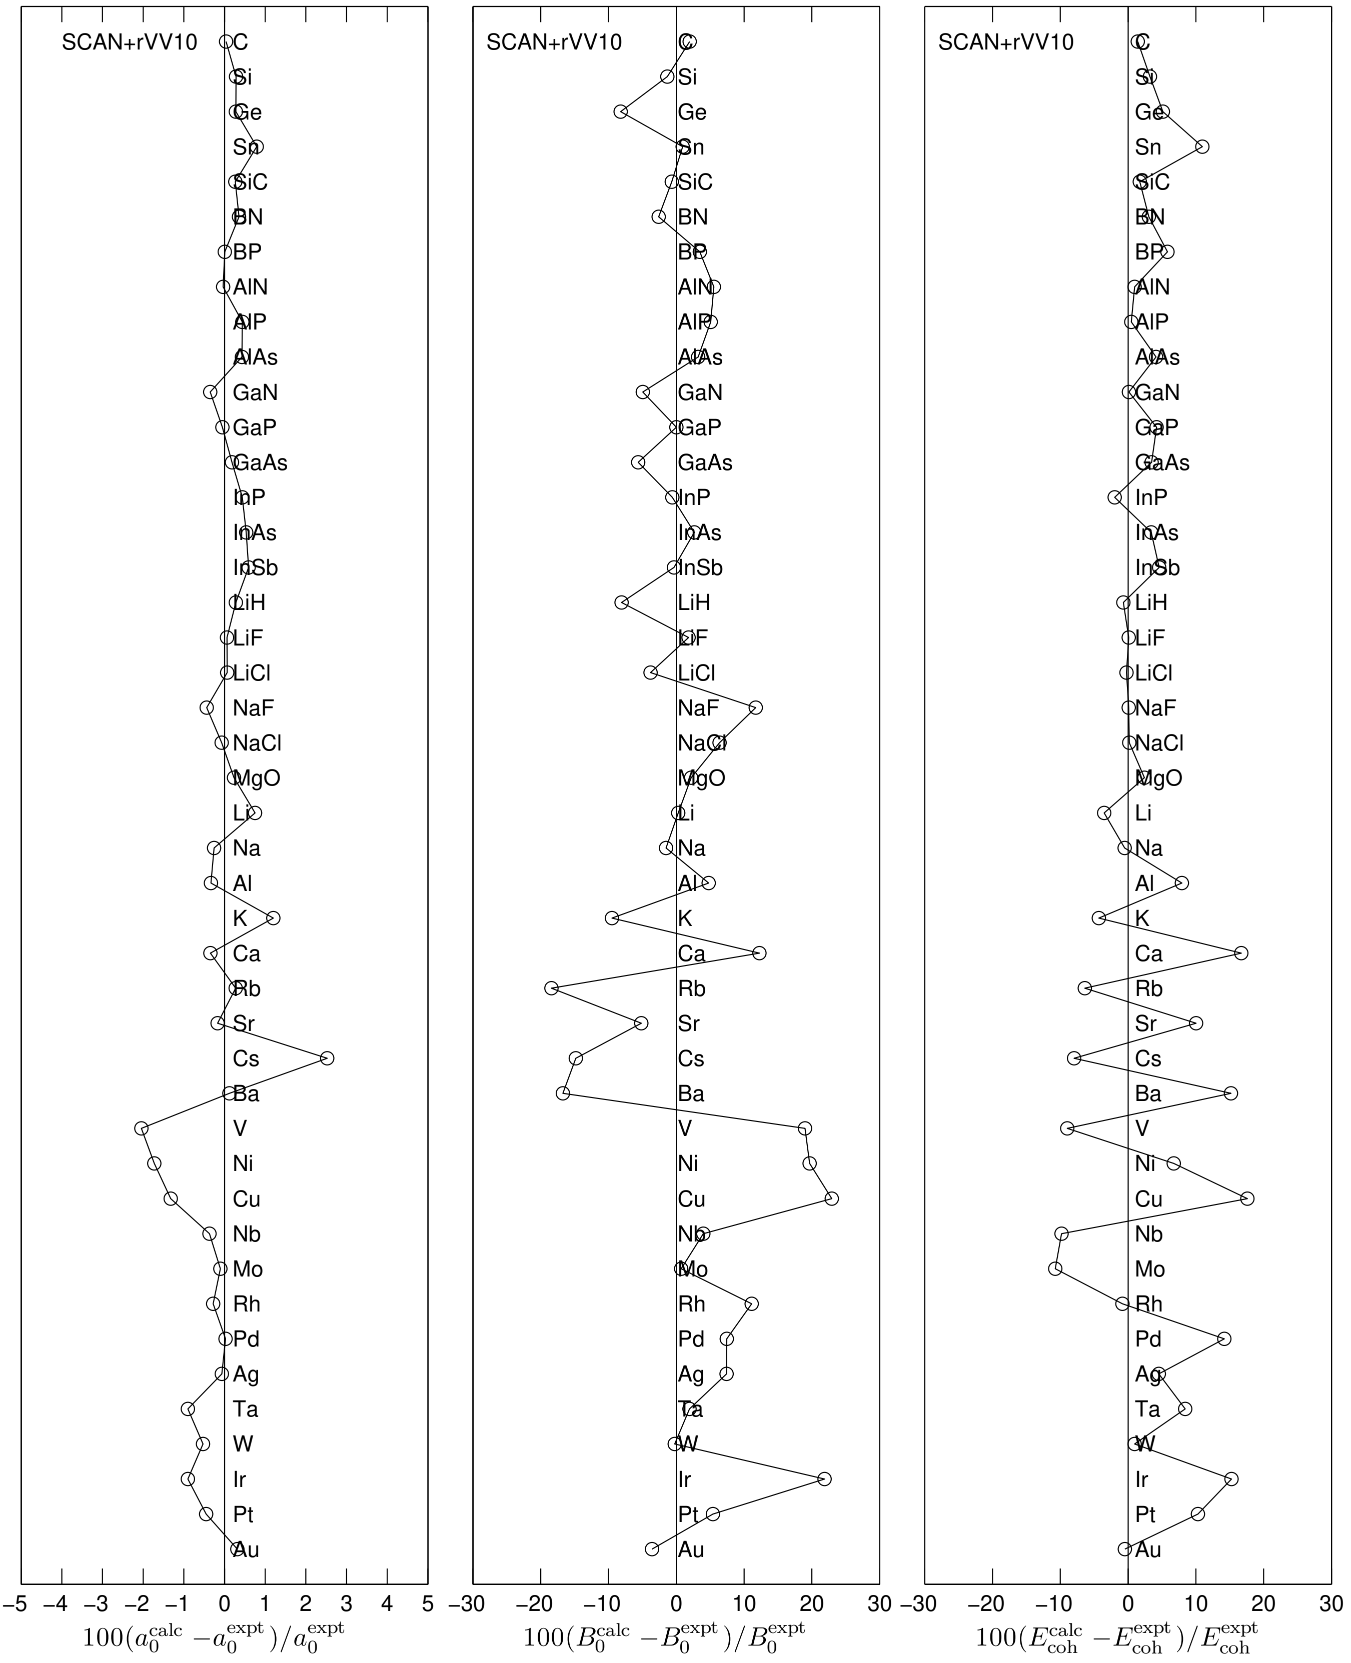


FIG. S6. Relative error (in %) in the calculated lattice constants $a_0$ (left), bulk modulus $B_0$ (middle), and cohesive energy $E_{\mathrm{coh}}$ (right) with respect to the experimental values.

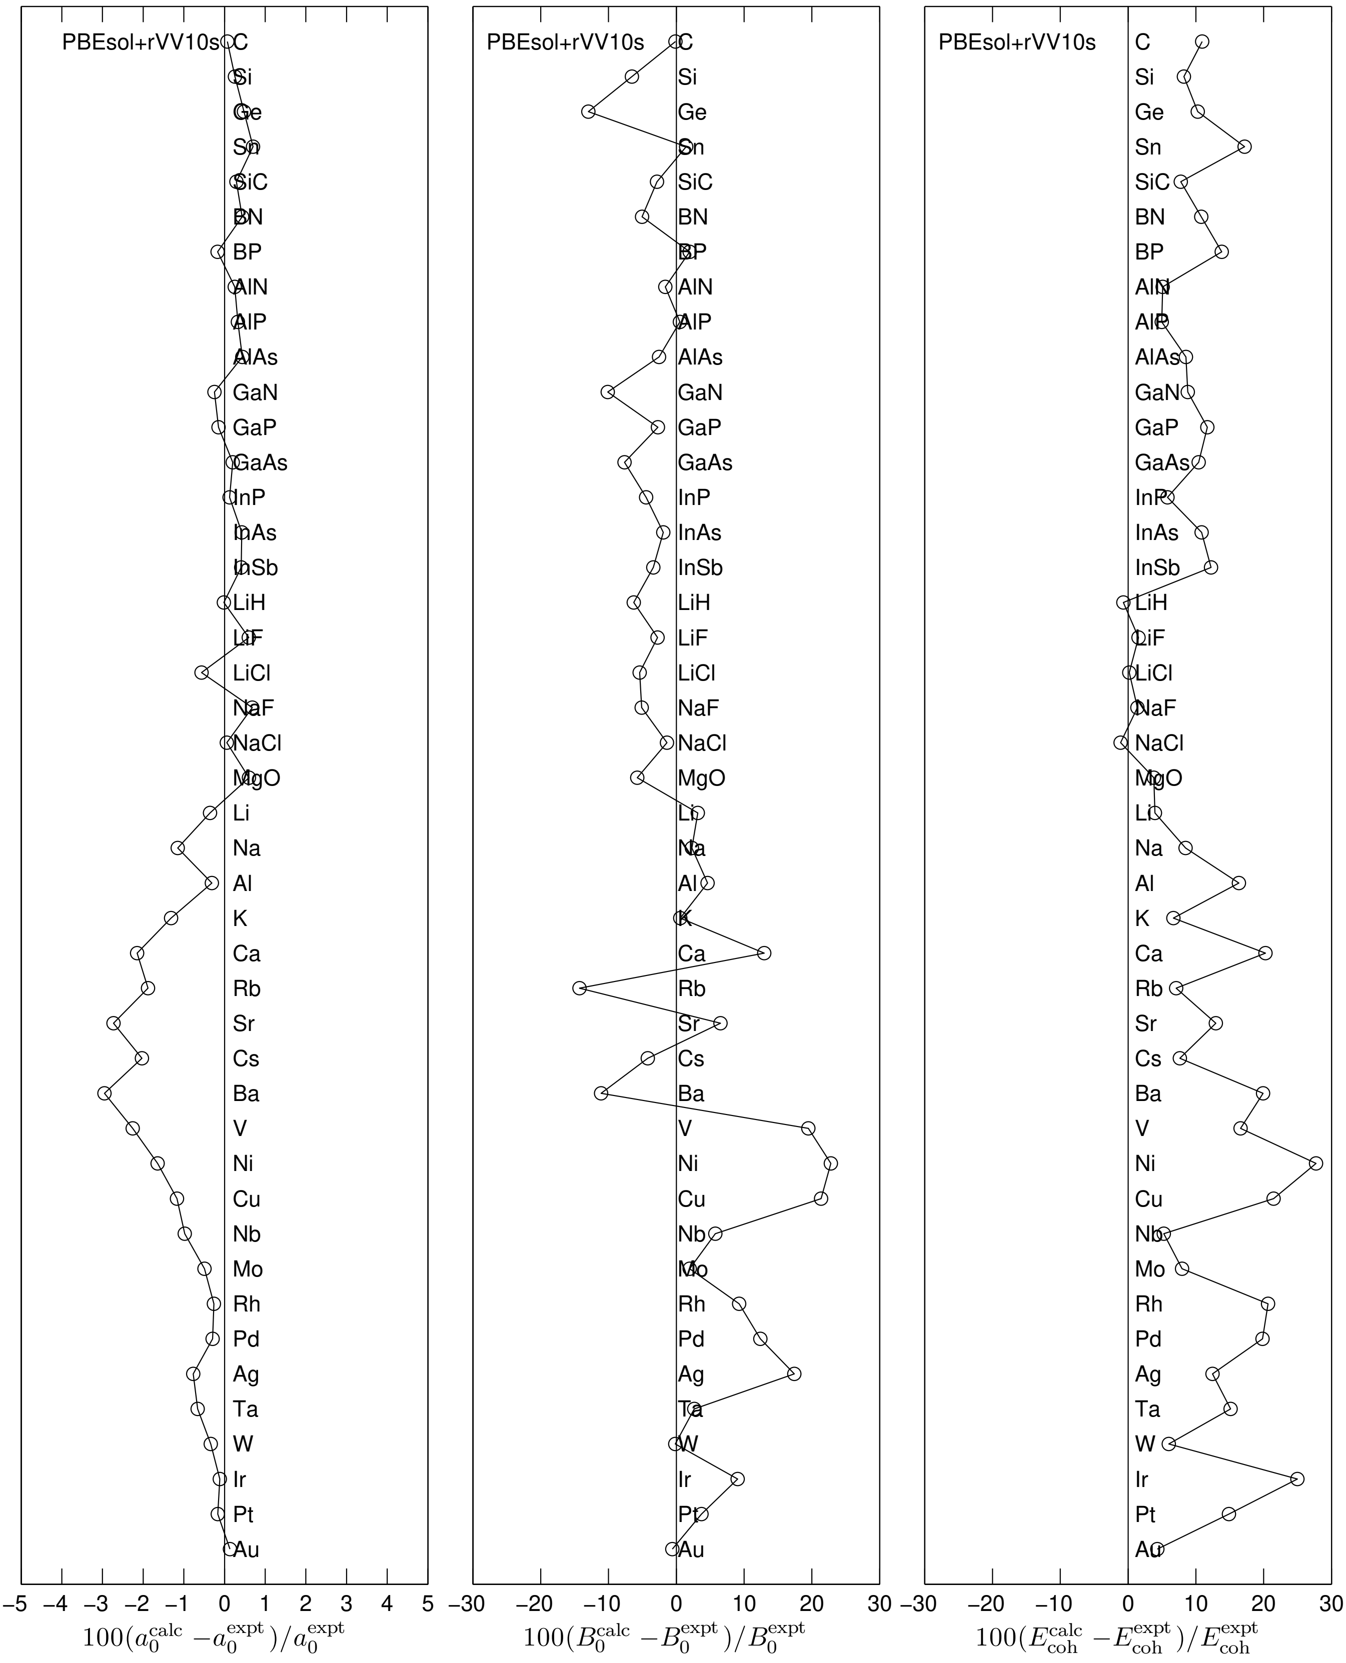


FIG. S7. Relative error (in %) in the calculated lattice constants $a_0$ (left), bulk modulus $B_0$ (middle), and cohesive energy $E_{\rm coh}$ (right) with respect to the experimental values.

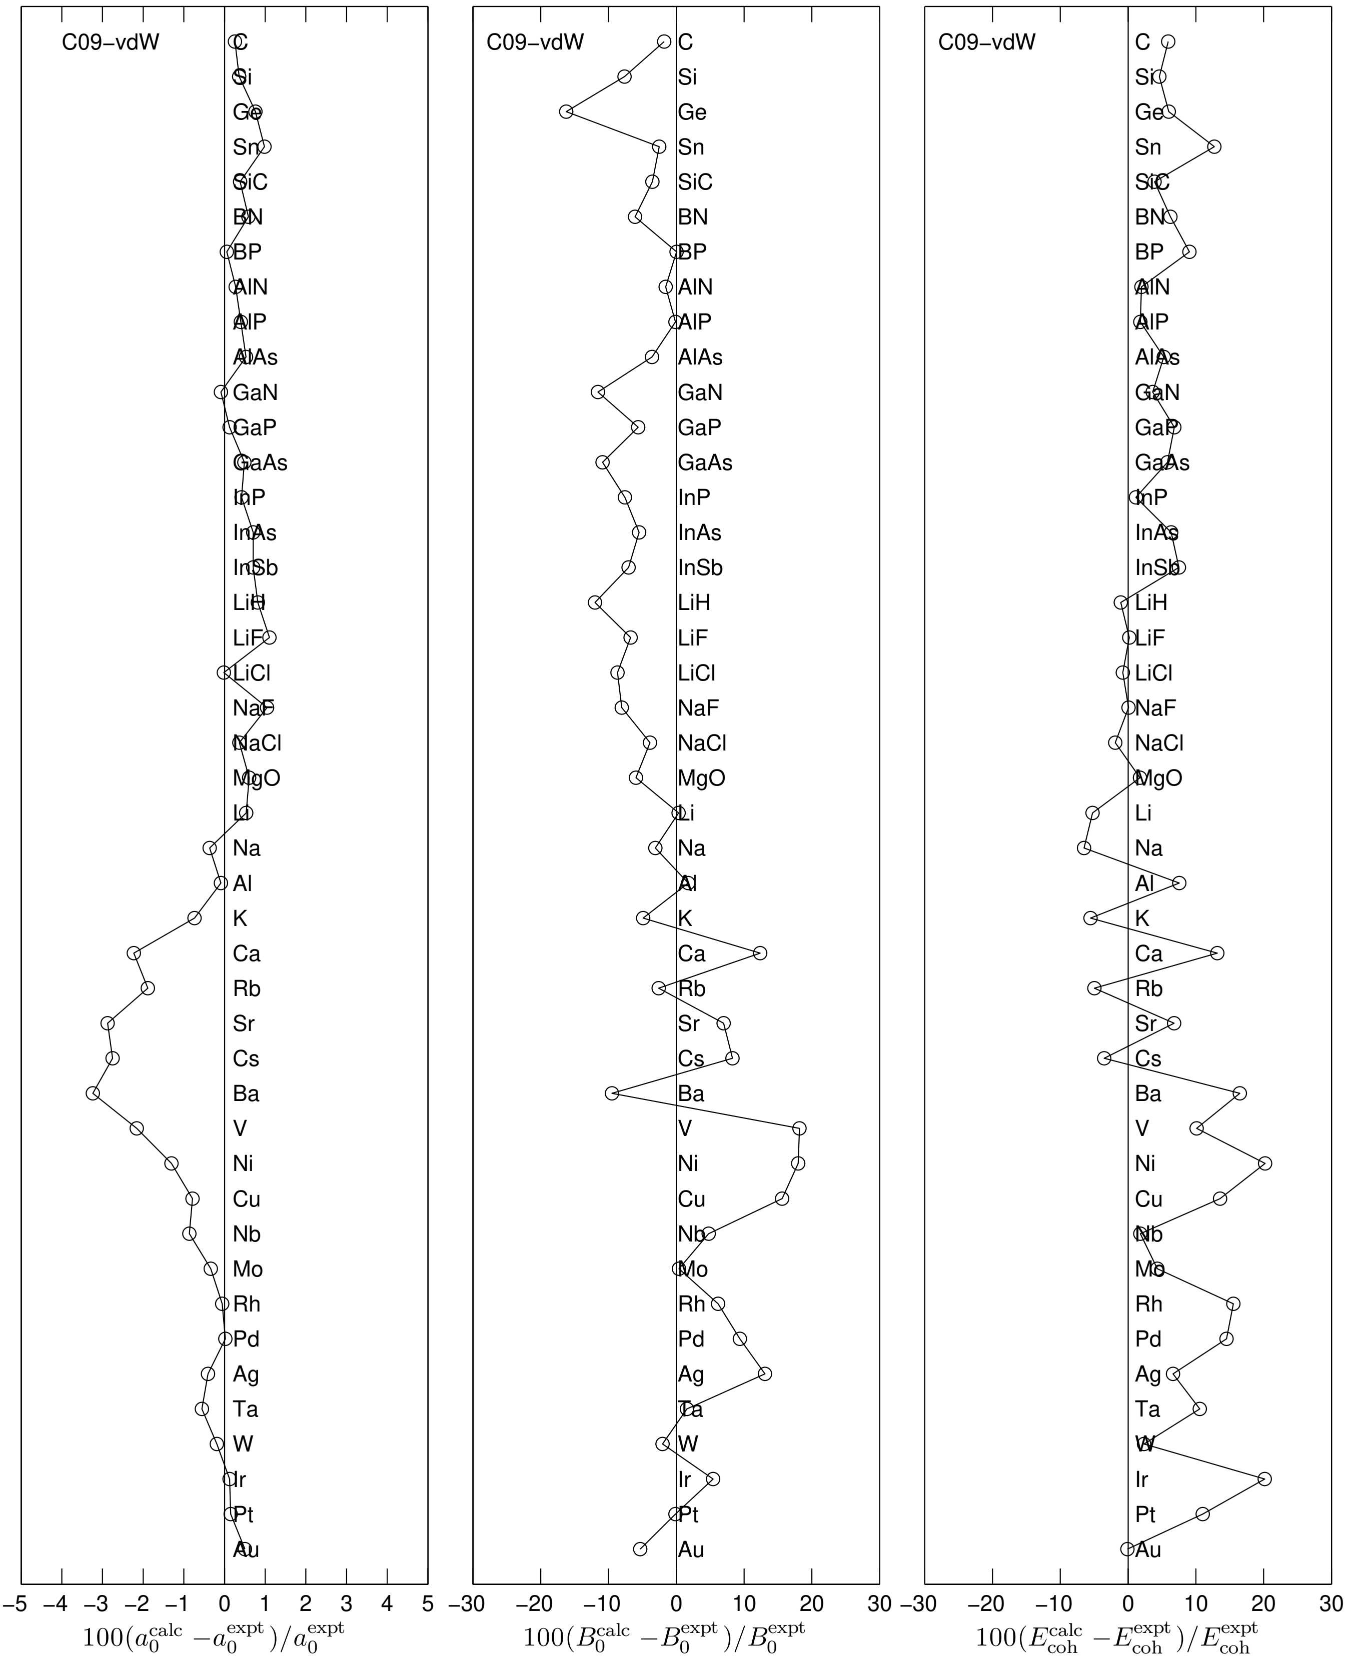


FIG. S8. Relative error (in %) in the calculated lattice constants $a_0$ (left), bulk modulus $B_0$ (middle), and cohesive energy $E_{\rm coh}$ (right) with respect to the experimental values.

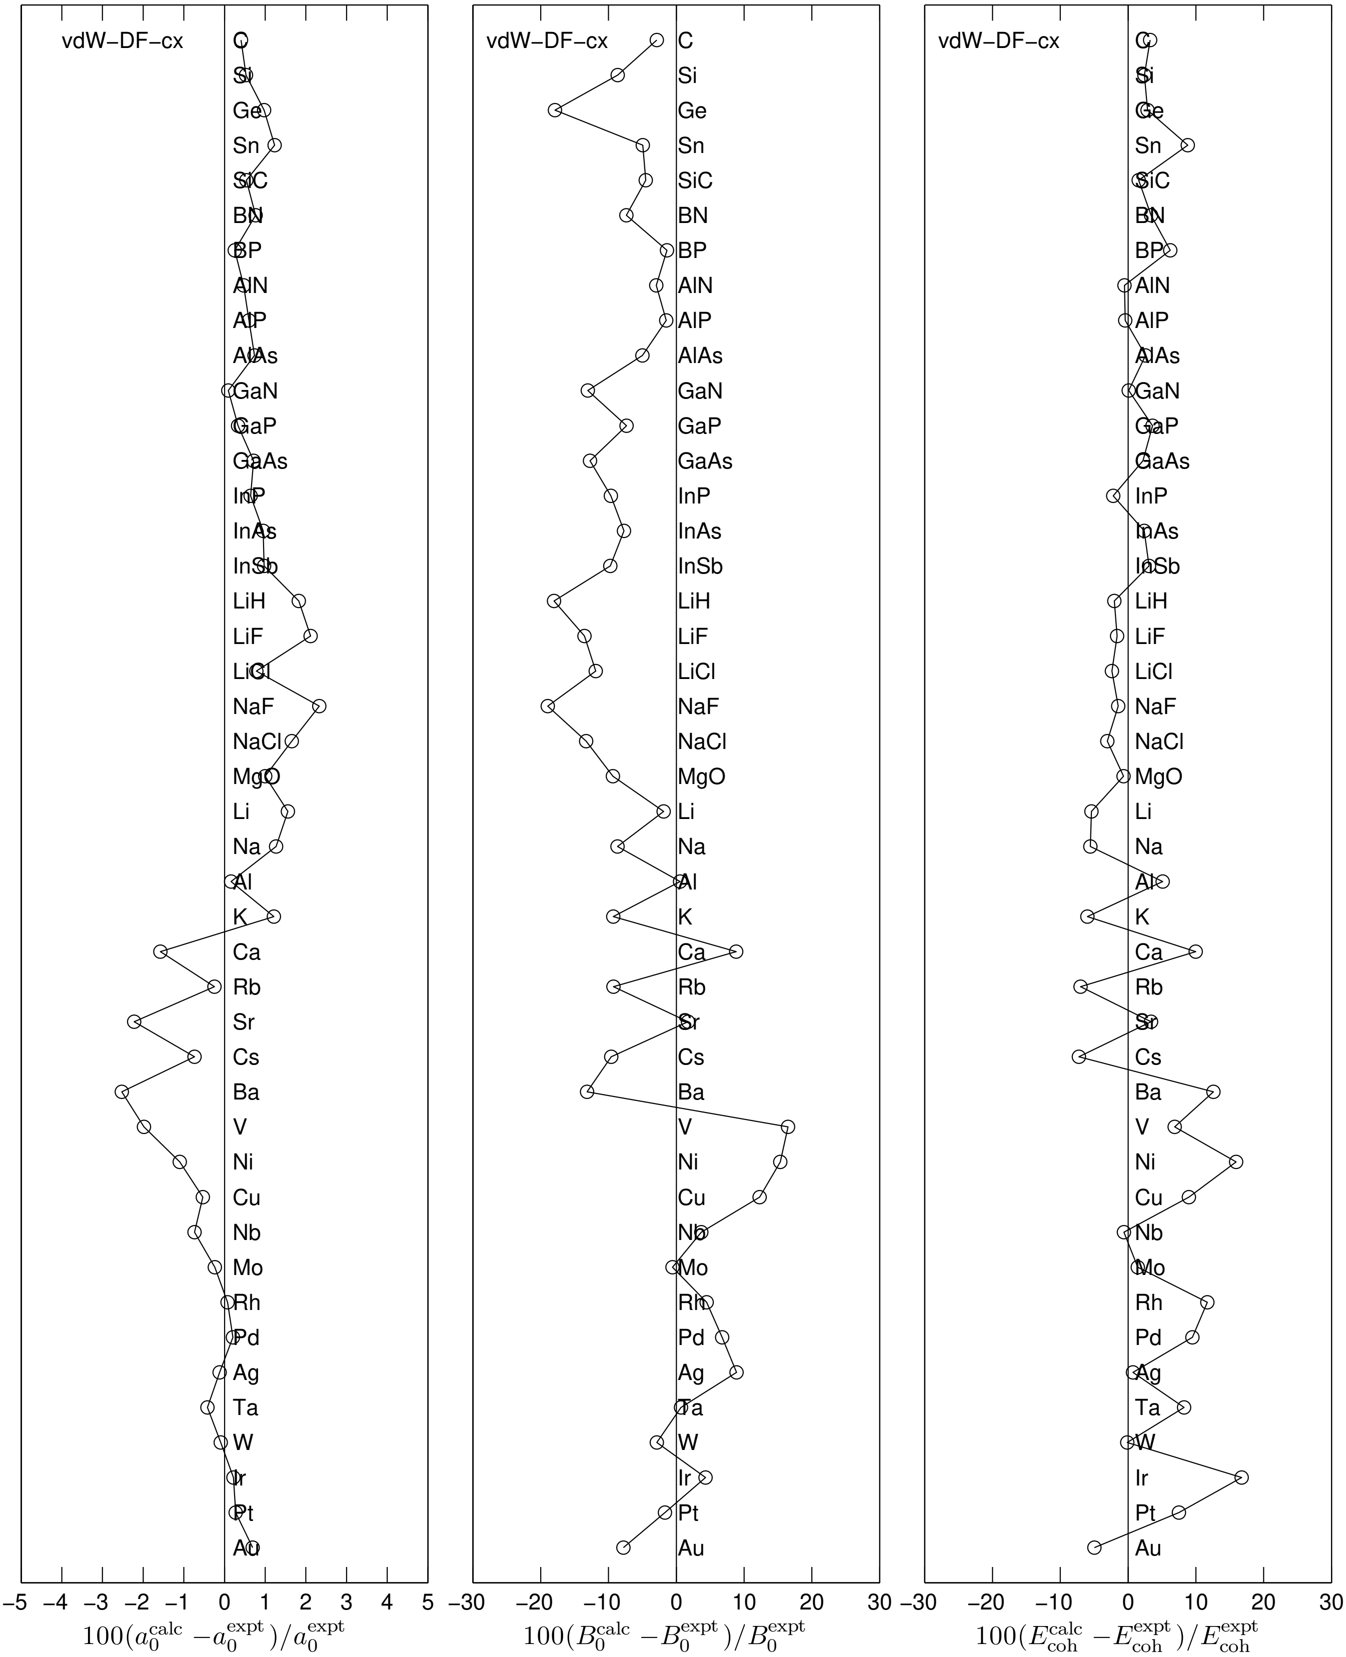


FIG. S9. Relative error (in %) in the calculated lattice constants $a_0$ (left), bulk modulus $B_0$ (middle), and cohesive energy $E_{\rm coh}$ (right) with respect to the experimental values.

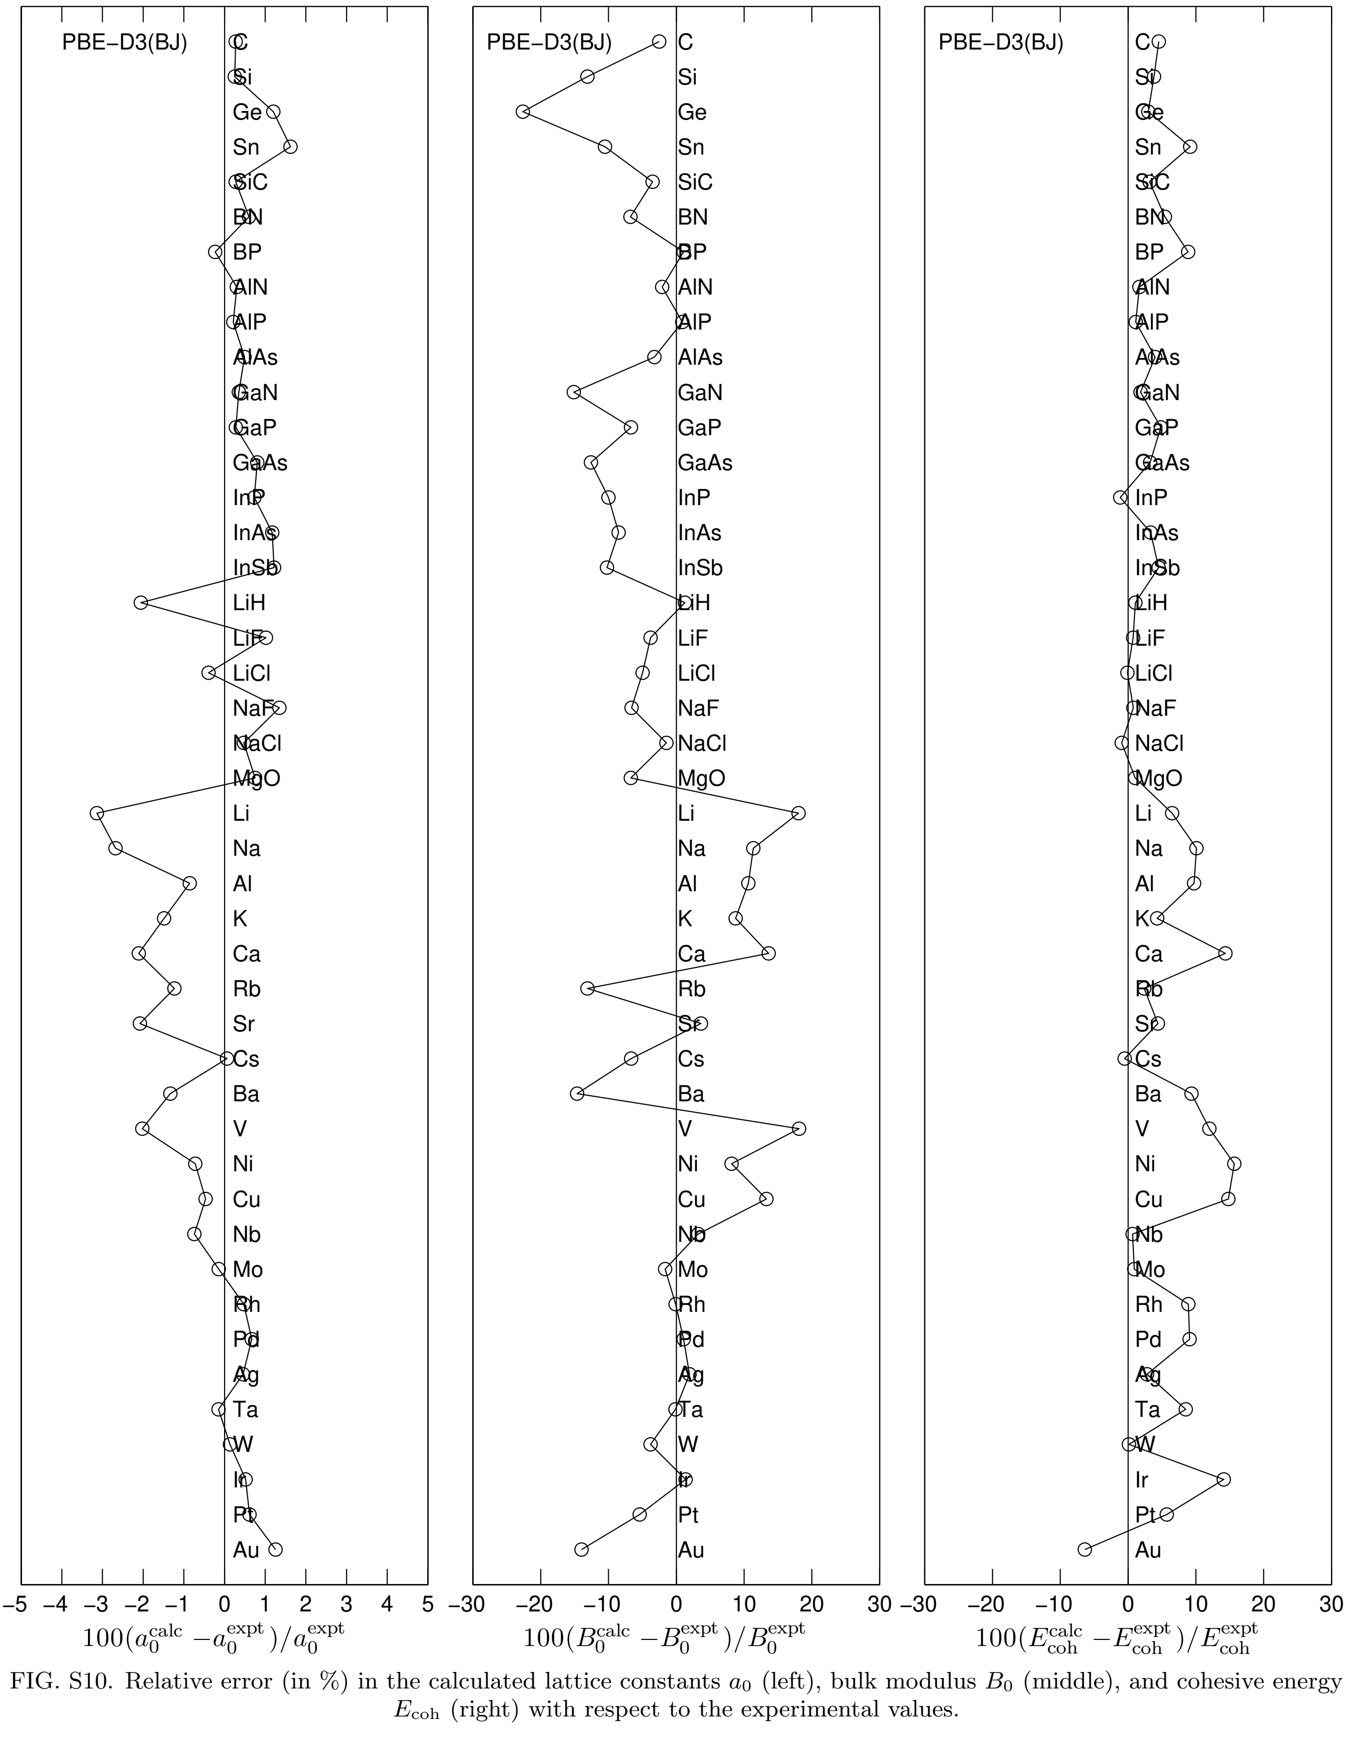


FIG. S10. Relative error (in %) in the calculated lattice constants $a_0$ (left), bulk modulus $B_0$ (middle), and cohesive energy $E_{\rm coh}$ (right) with respect to the experimental values.

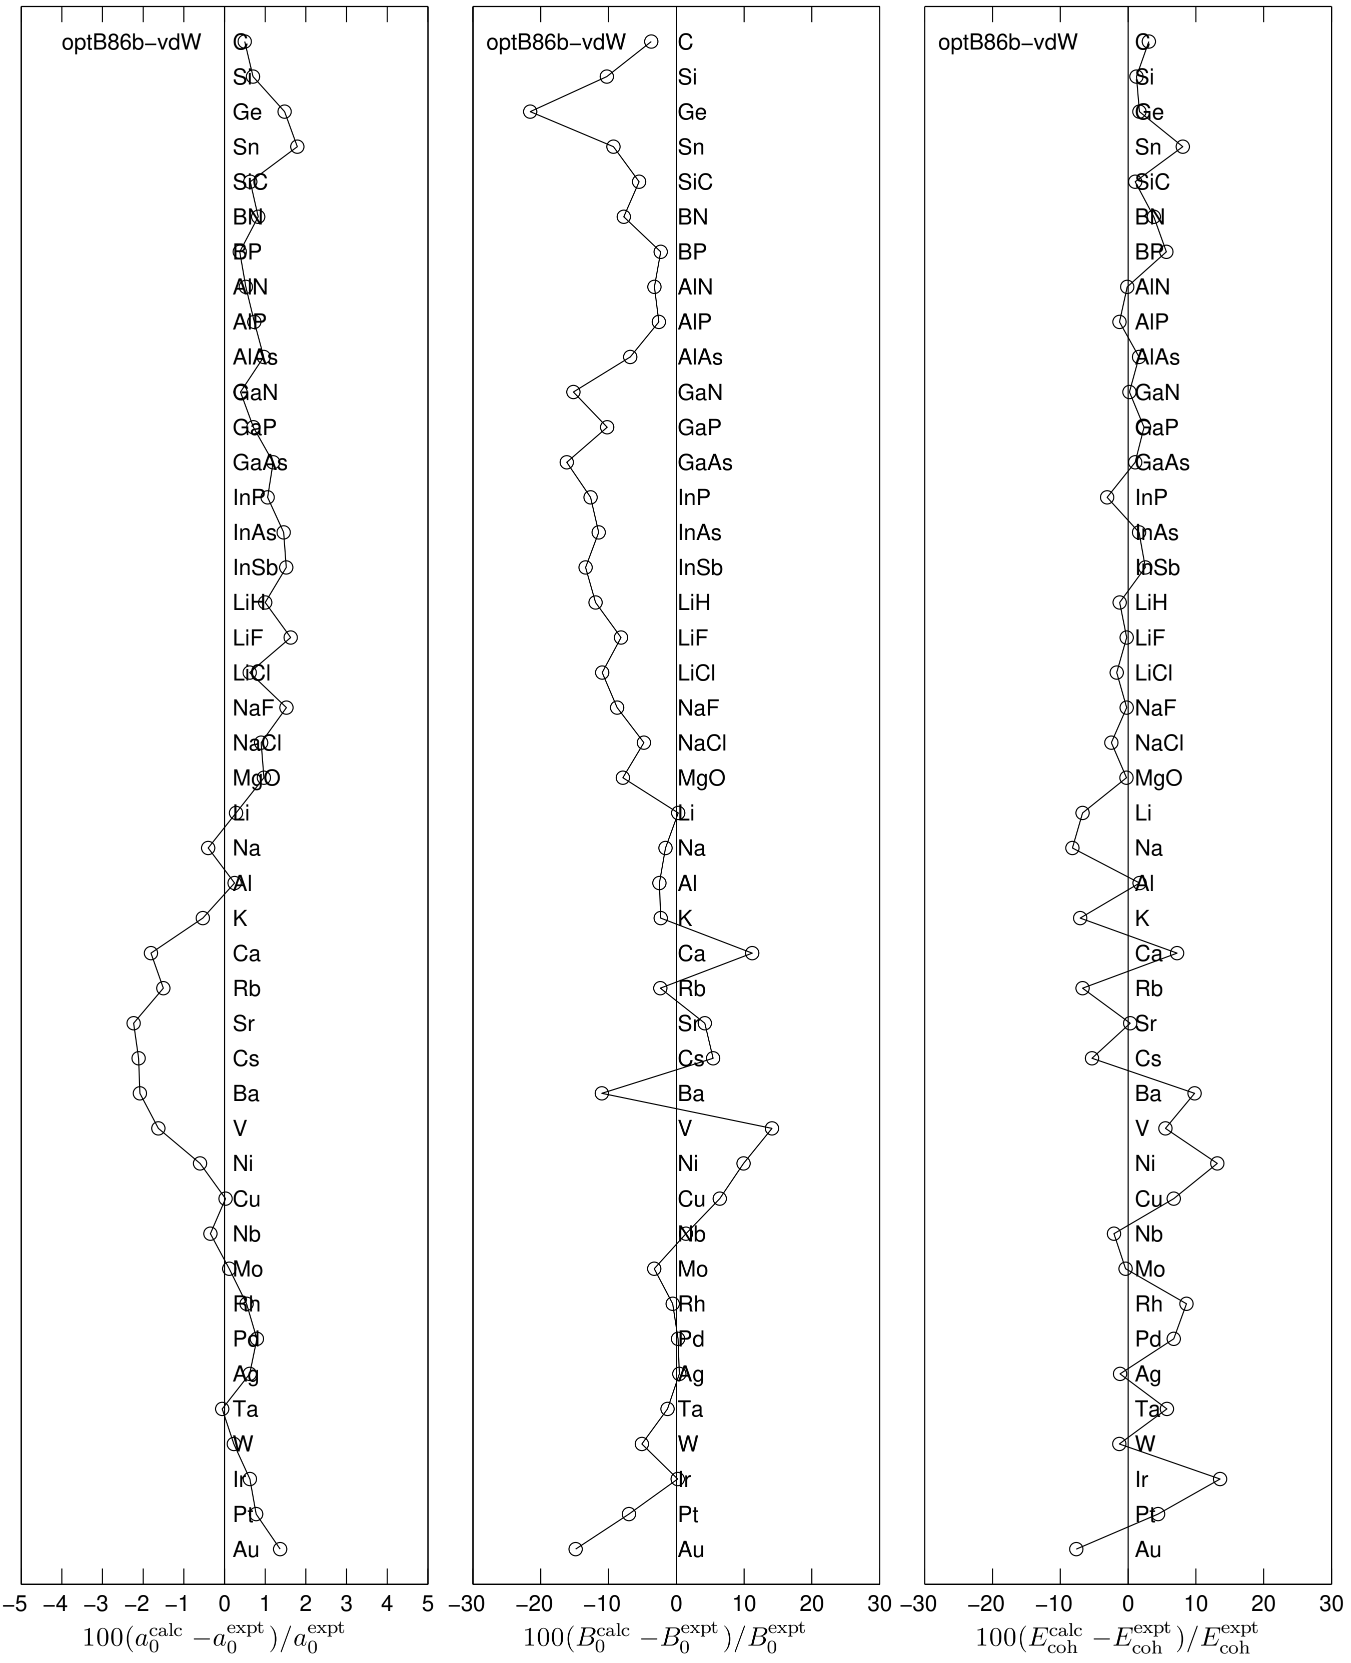


FIG. S11. Relative error (in %) in the calculated lattice constants $a_0$ (left), bulk modulus $B_0$ (middle), and cohesive energy $E_{\rm coh}$ (right) with respect to the experimental values.

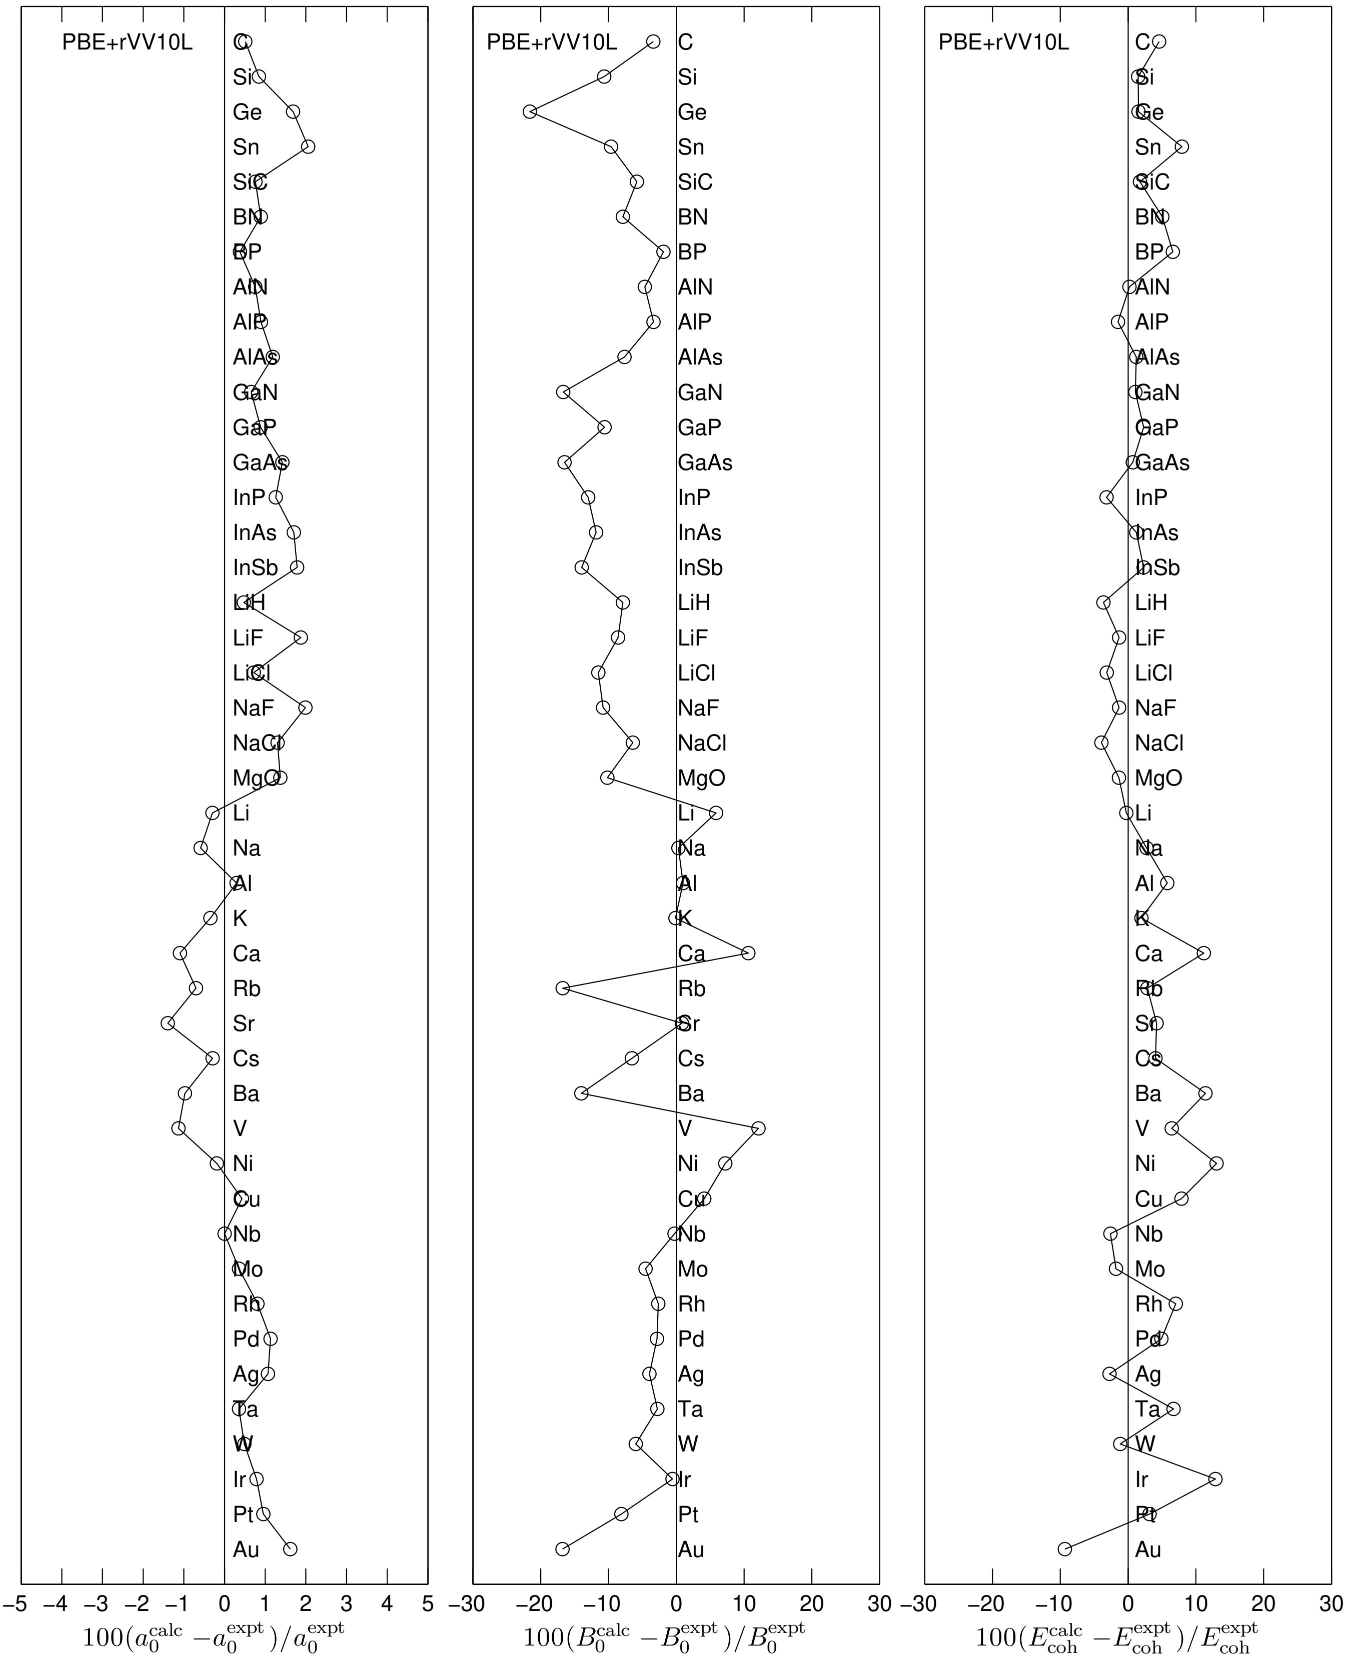


FIG. S12. Relative error (in %) in the calculated lattice constants $a_0$ (left), bulk modulus $B_0$ (middle), and cohesive energy $E_{\rm coh}$ (right) with respect to the experimental values.

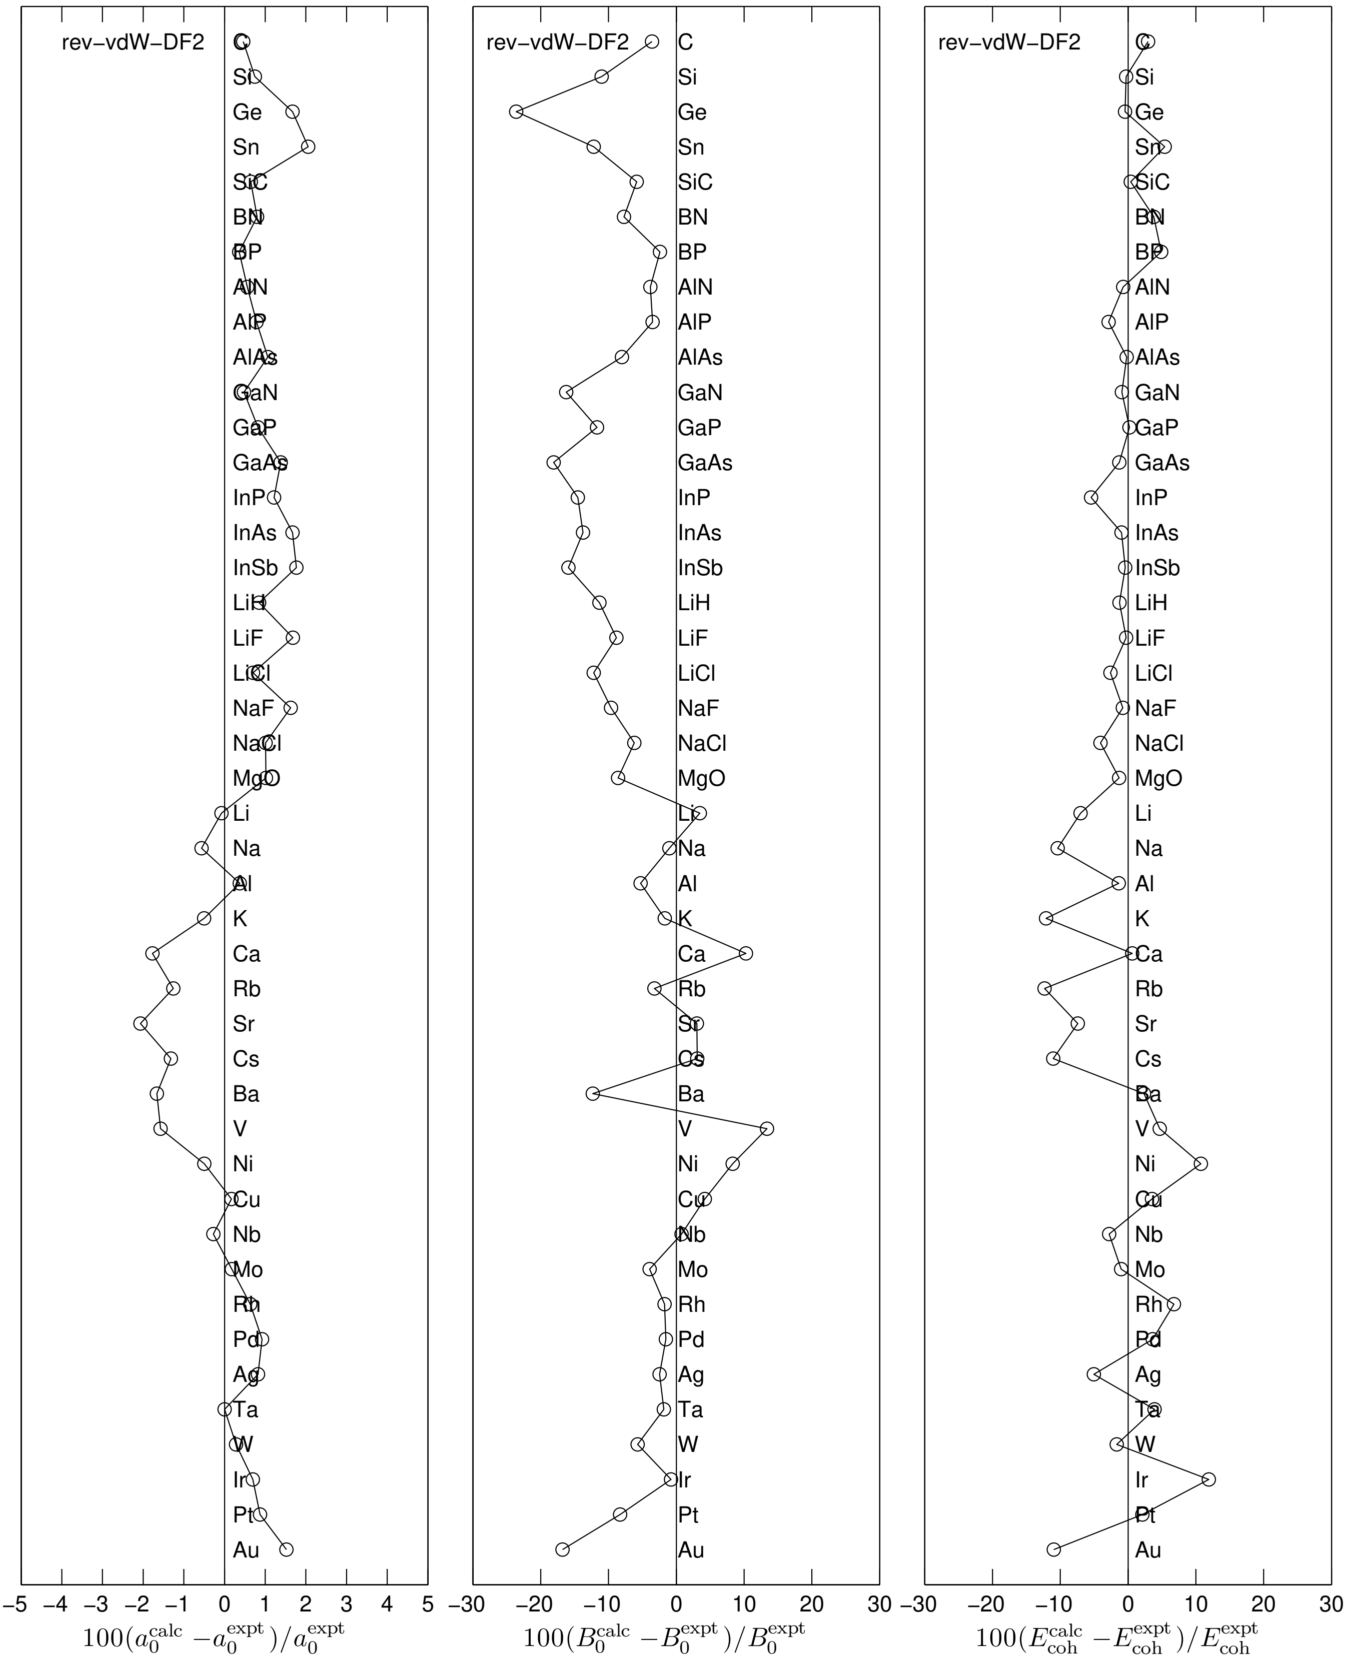


FIG. S13. Relative error (in %) in the calculated lattice constants $a_0$ (left), bulk modulus $B_0$ (middle), and cohesive energy $E_{\rm coh}$ (right) with respect to the experimental values.

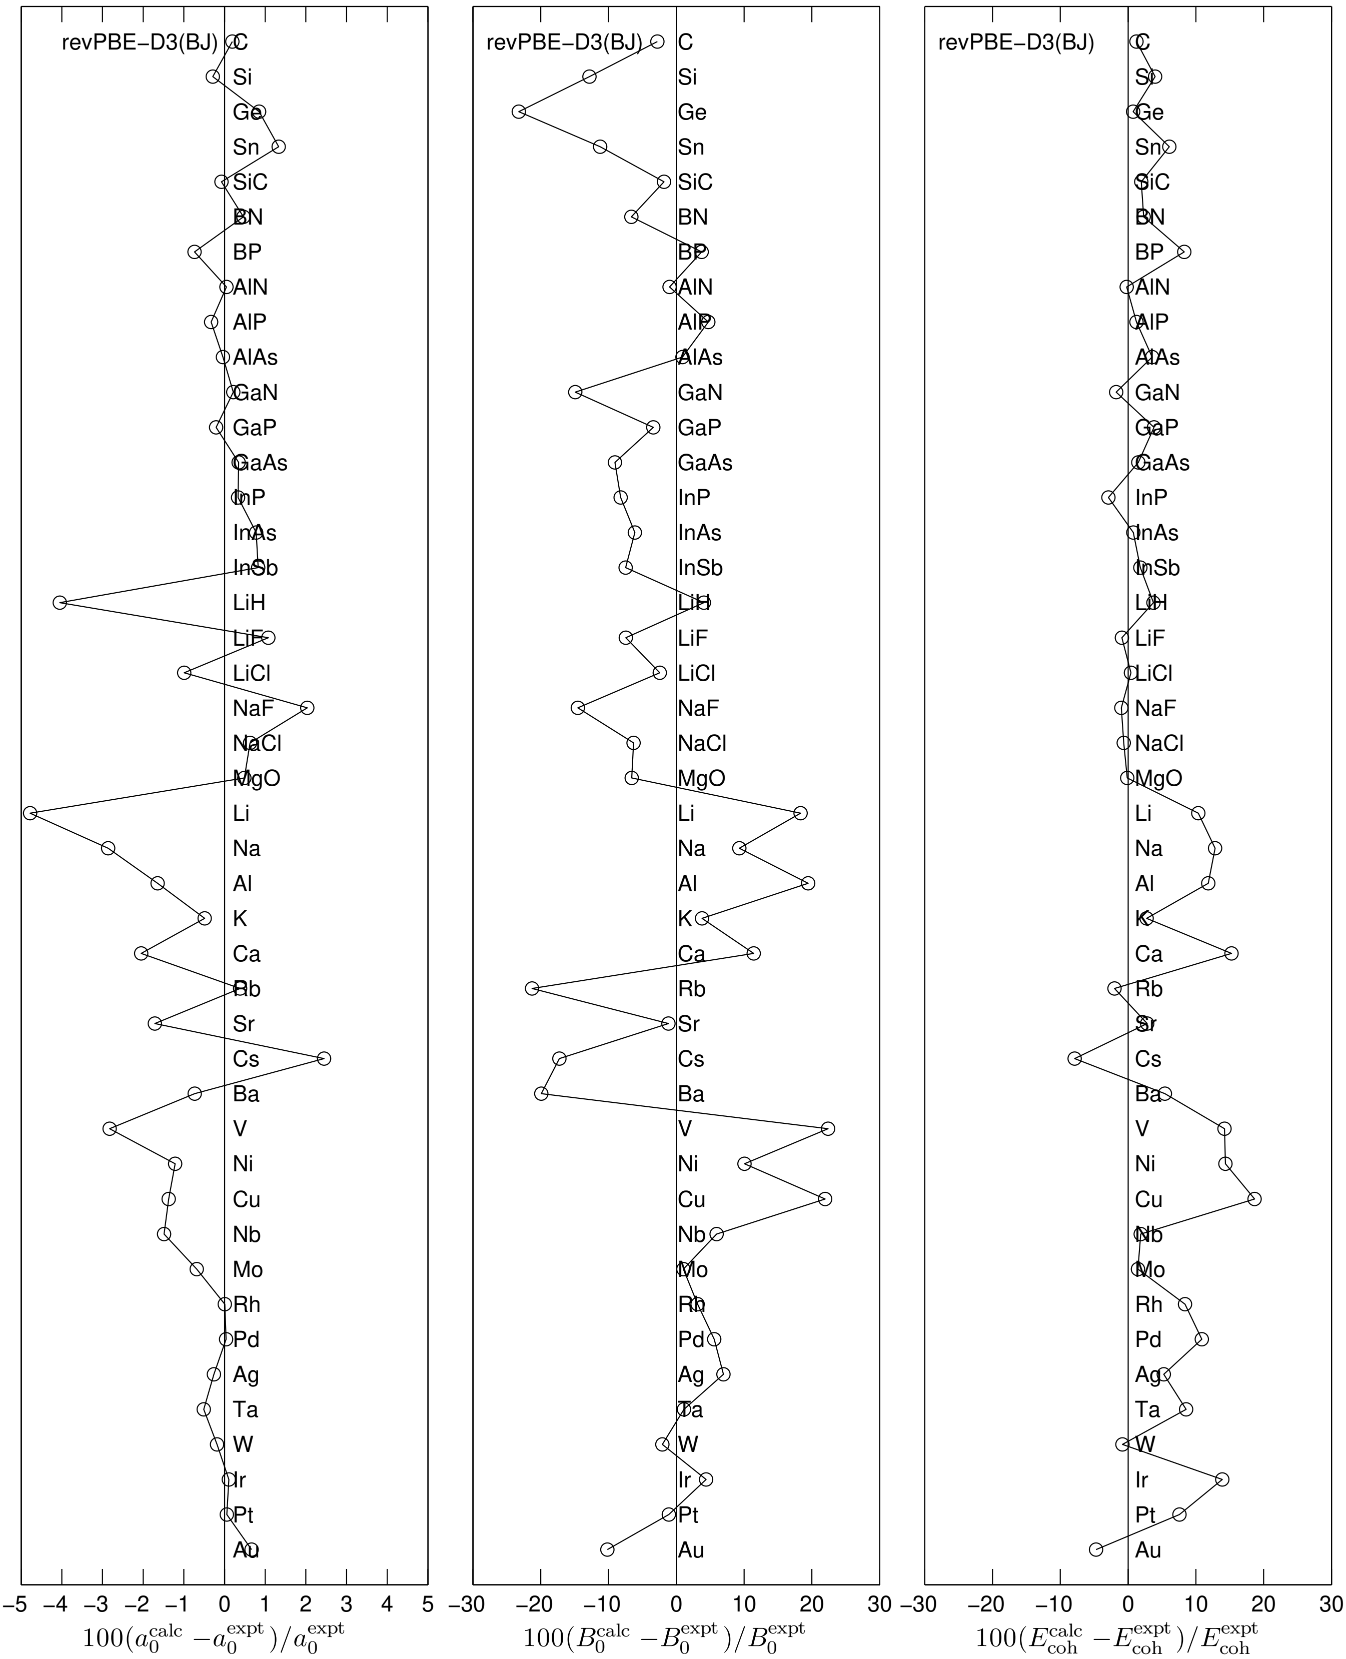


FIG. S14. Relative error (in %) in the calculated lattice constants $a_0$ (left), bulk modulus $B_0$ (middle), and cohesive energy $E_{\rm coh}$ (right) with respect to the experimental values.

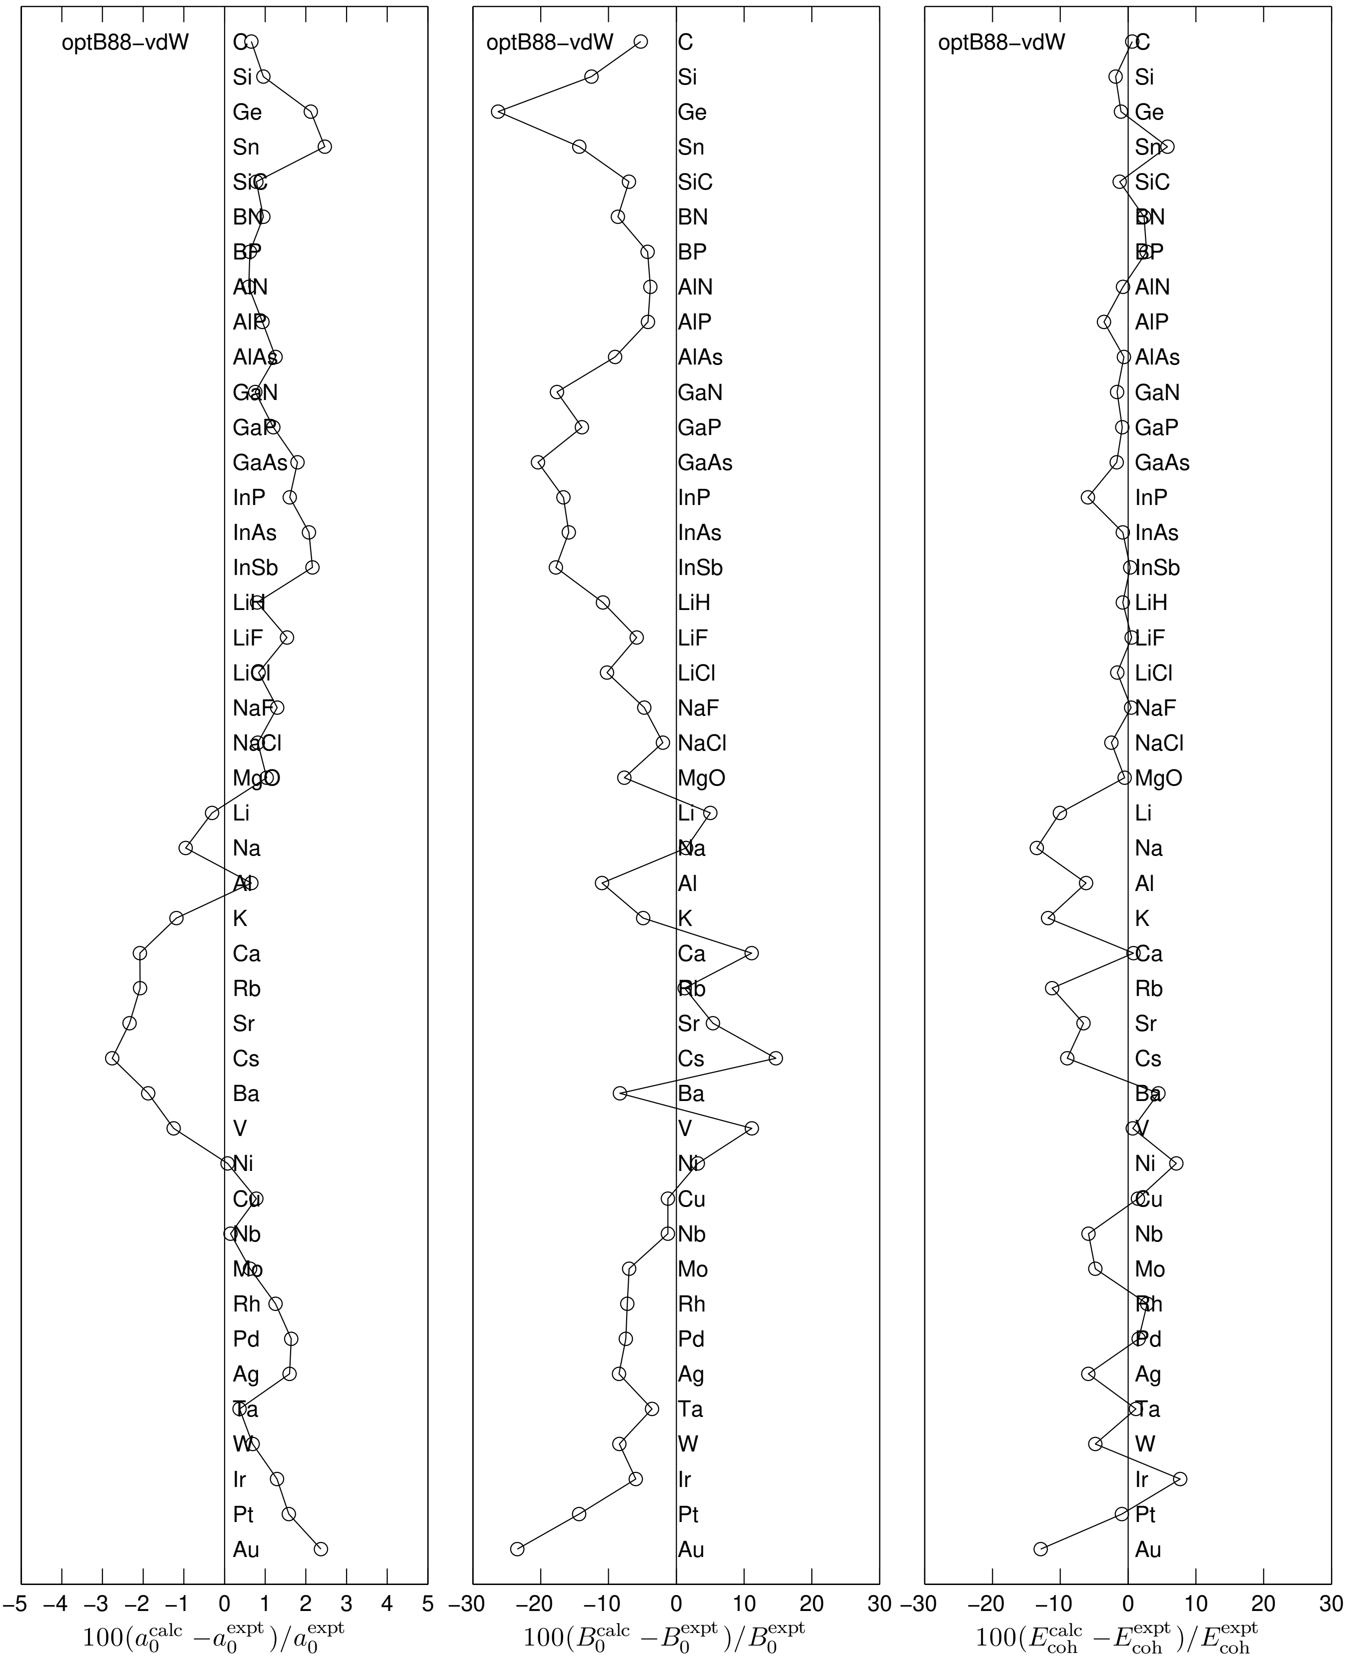


FIG. S15. Relative error (in %) in the calculated lattice constants $a_0$ (left), bulk modulus $B_0$ (middle), and cohesive energy $E_{\mathrm{coh}}$ (right) with respect to the experimental values.

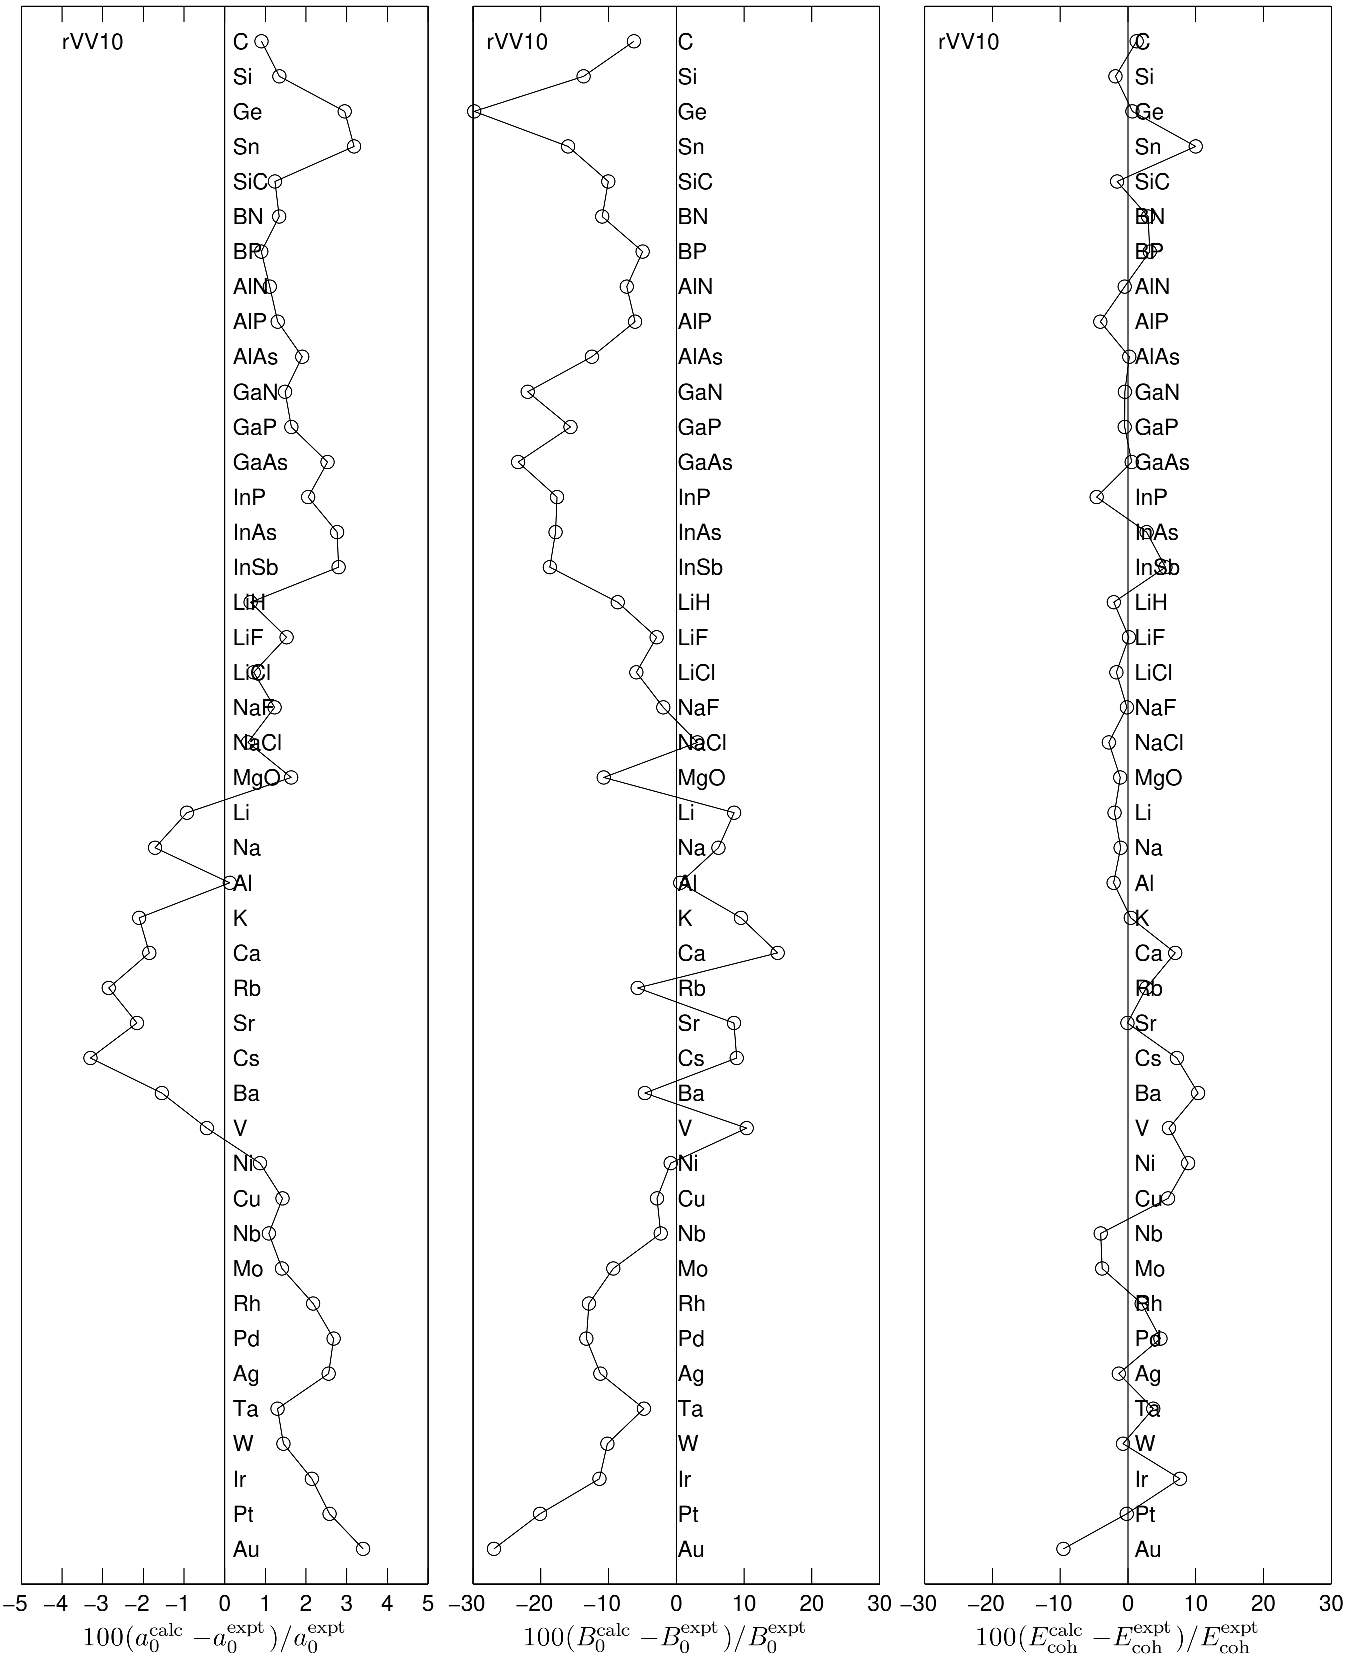


FIG. S16. Relative error (in %) in the calculated lattice constants $a_0$ (left), bulk modulus $B_0$ (middle), and cohesive energy $E_{\text{coh}}$ (right) with respect to the experimental values.

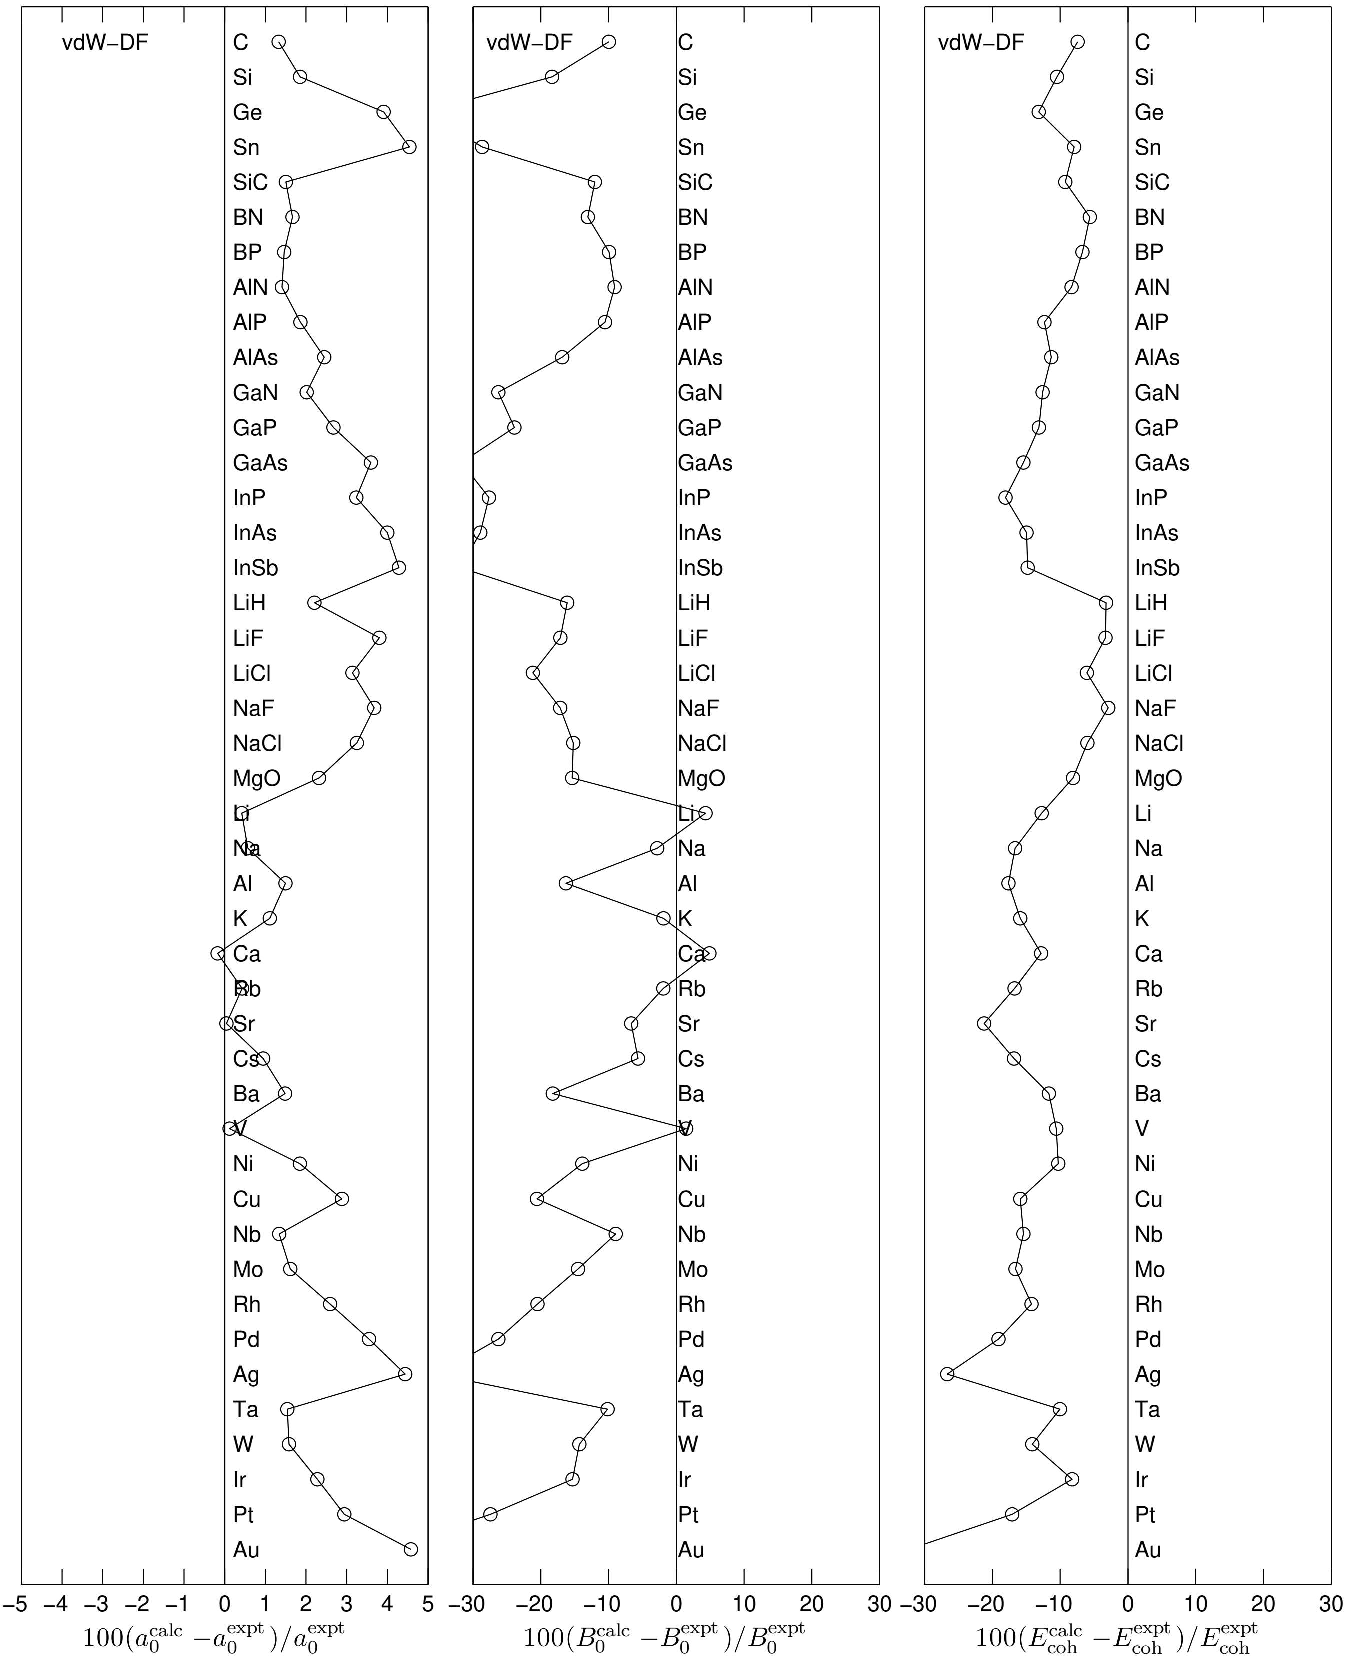


FIG. S17. Relative error (in %) in the calculated lattice constants $a_0$ (left), bulk modulus $B_0$ (middle), and cohesive energy $E_{\mathrm{coh}}$ (right) with respect to the experimental values.

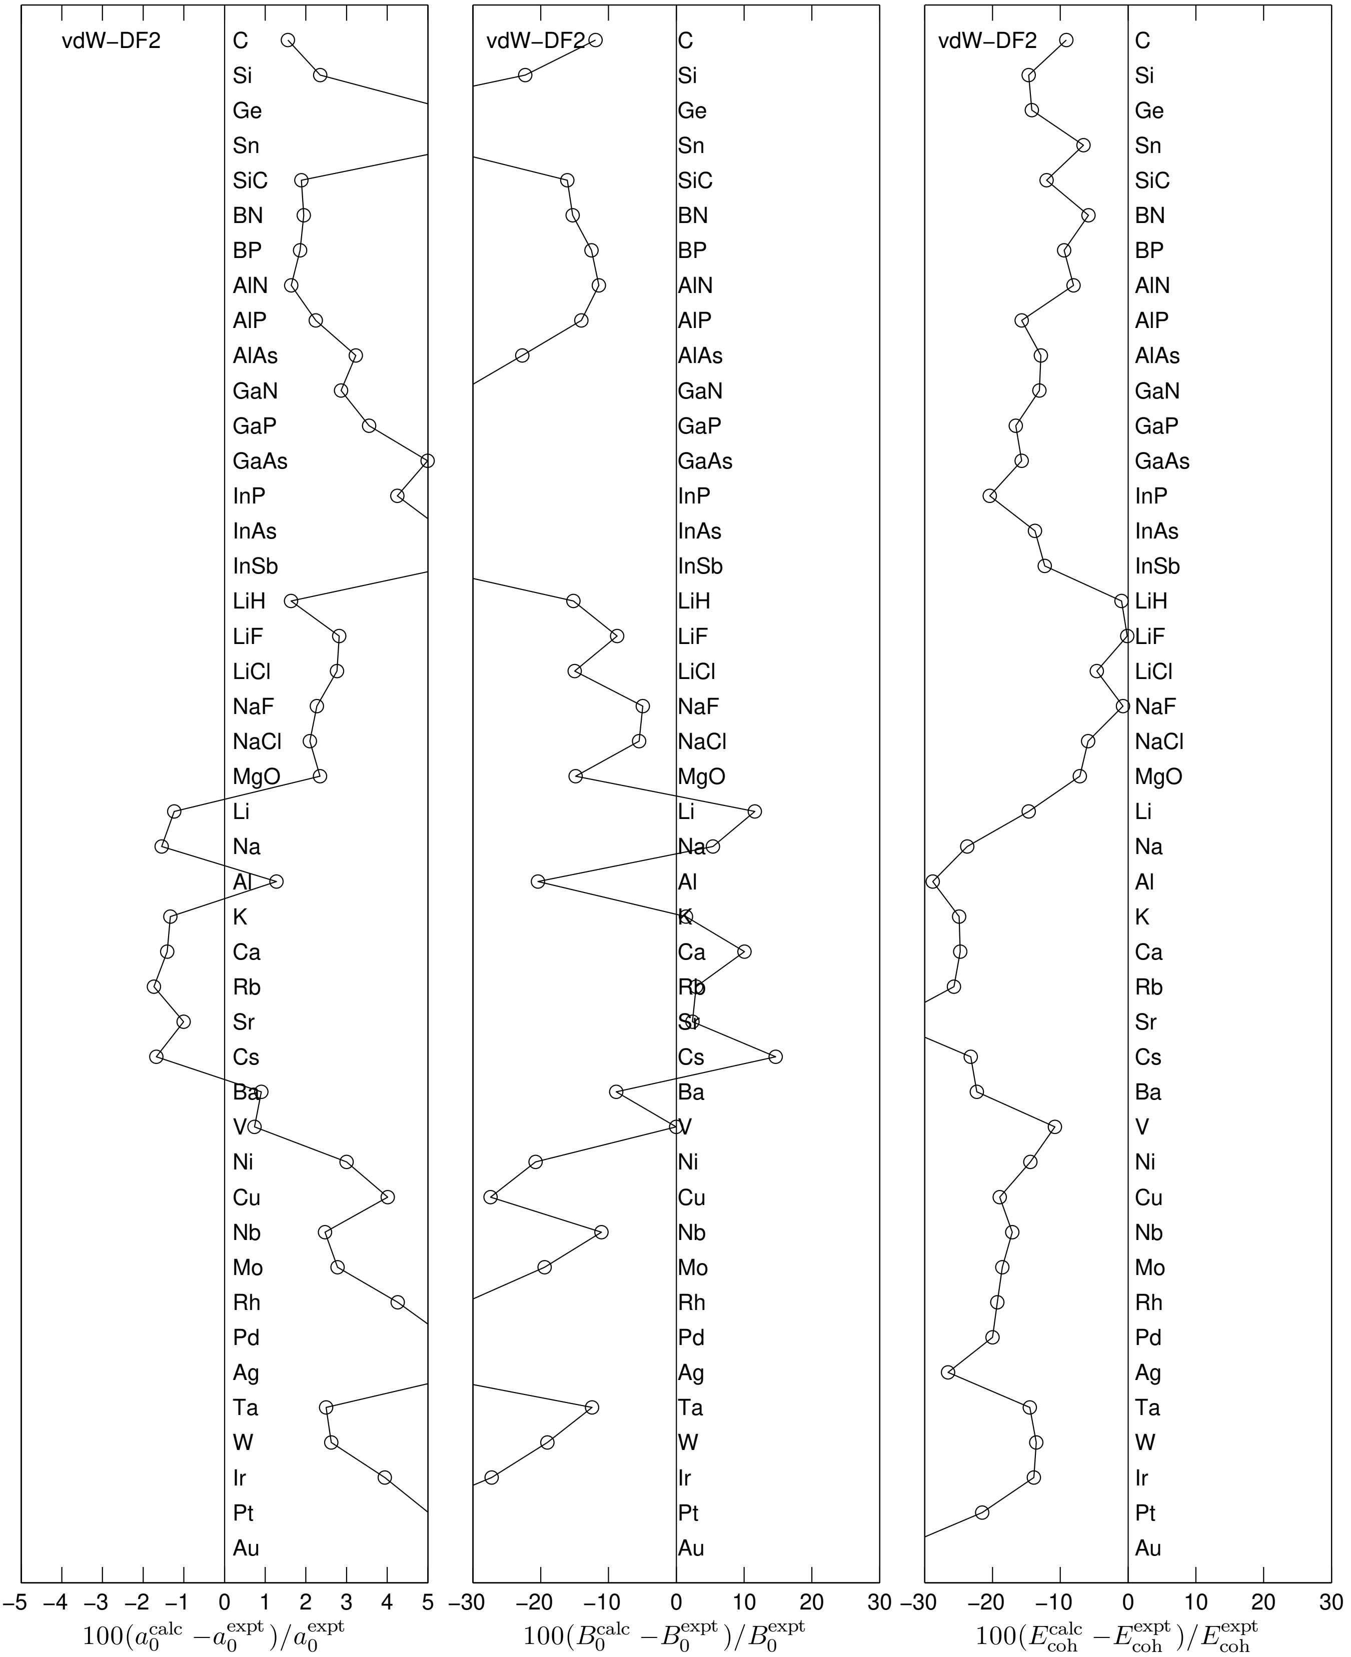


FIG. S18. Relative error (in %) in the calculated lattice constants $a_0$ (left), bulk modulus $B_0$ (middle), and cohesive energy $E_{\mathrm{coh}}$ (right) with respect to the experimental values.

TABLE S10. Atomization energy (in eV) for the molecules of the AE6 test set[1] obtained with four functionals and with different codes. The vdW-DF2, optB88-vdW, and rev-vdW-DF2 calculations were done using the non-spin-polarized version of the DRSLL and LMKLL kernels. The error (in %) with respect to experiment[1] is indicated in parenthesis. The units of the MRE and MARE are %.

| | $SiH_4$ | SiO | $S_2$ | $C_3H_4$ | $C_2H_2O_2$ | $C_4H_8$ | ME | MAE | MRE | MARE |
|---|---|---|---|---|---|---|---|---|---|---|
| | | | | | PBE | | | | | |
| CP2K[a] | 13.58 (-3) | 8.50 (2) | 4.98 (13) | 31.27 (2) | 28.84 (5) | 50.64 (2) | 0.54 | 0.67 | 3.5 | 4.5 |
| VASP[a] | 13.57 (-3) | 8.45 (1) | 4.99 (13) | 31.20 (2) | 28.61 (4) | 50.53 (1) | 0.46 | 0.60 | 3.2 | 4.2 |
| VASP[b] | 13.59 (-3) | 8.47 (2) | 4.98 (13) | 31.13 (2) | 28.53 (4) | 50.46 (1) | 0.43 | 0.56 | 3.2 | 4.1 |
| | | | | | vdW-DF2 | | | | | |
| CP2K[a] | 14.20 (2) | 8.41 (1) | 4.44 (1) | 30.50 (0) | 27.63 (1) | 49.27 (-1) | -0.02 | 0.19 | 0.4 | 0.9 |
| VASP[a] | 14.17 (1) | 8.37 (0) | 4.45 (1) | 30.45 (0) | 27.51 (0) | 49.16 (-1) | -0.08 | 0.18 | 0.2 | 0.8 |
| VASP[b] | 8.91 (-36) | 8.30 (0) | 4.38 (-1) | 29.95 (-2) | 26.95 (-2) | 54.27 (9) | -0.30 | 1.78 | -5.4 | 8.4 |
| | | | | | optB88-vdW | | | | | |
| CP2K[a] | 14.50 (4) | 8.73 (5) | 5.00 (13) | 31.63 (4) | 29.07 (6) | 51.54 (3) | 0.98 | 0.98 | 5.8 | 5.8 |
| VASP[a] | 14.44 (3) | 8.92 (7) | 5.14 (17) | 31.97 (5) | 29.64 (8) | 51.96 (4) | 1.25 | 1.25 | 7.3 | 7.3 |
| VASP[b] | 13.46 (-4) | 8.06 (-3) | 4.55 (3) | 29.07 (-5) | 26.52 (-3) | 47.30 (-5) | -0.94 | 0.98 | -2.8 | 3.9 |
| | | | | | rev-vdW-DF2 | | | | | |
| CP2K[a] | 14.42 (3) | 8.77 (5) | 5.05 (15) | 31.87 (4) | 29.39 (7) | 51.92 (4) | 1.14 | 1.14 | 6.4 | 6.4 |
| VASP[a] | 14.37 (3) | 8.95 (7) | 5.23 (19) | 31.78 (4) | 29.62 (8) | 51.77 (4) | 1.19 | 1.19 | 7.4 | 7.4 |
| VASP[b] | 14.39 (3) | 8.77 (5) | 5.08 (15) | 31.58 (3) | 29.06 (6) | 55.39 (11) | 1.62 | 1.62 | 7.3 | 7.3 |
| | | | | | Reference | | | | | |
| | 13.98 | 8.33 | 4.41 | 30.56 | 27.46 | 49.83 | | | | |

[a] This work.
[b] Results from Ref. 2.


[1] B. J. Lynch and D. G. Truhlar, J. Phys. Chem. A **107**, 8996 (2003); **108**, 1460 (2004).
[2] M. Callsen and I. Hamada, Phys. Rev. B **91**, 195103 (2015); **95**, 039905(E) (2017).
